# Supplementary material for: A search for variable subdwarf B stars in TESS Full Frame Images -- I. Variable objects in the southern ecliptic hemisphere
Source: arXiv:2011.03465 ancillary file (2020-11-06)

Basic information of 11 spectroscopically classified eclipsing binaries. The table is followed by phased lightcurves of these targets.

| Gaia DR2                               | TIC        | Spec Type | G mag   | Sector | Period [d] | Remarks                               |
|----------------------------------------|------------|-----------|---------|--------|------------|---------------------------------------|
| <b>Primary and secondary eclipses:</b> |            |           |         |        |            |                                       |
| 4040428807982926336                    | 257415989  | B9II/III  | 8.1672  | 13     | 2.1238     | TYC 7390-2323-2 1" away               |
| 4054618662690377856                    | 1422846269 | B9V       | 10.0886 | 12     | 1.7862     | crowded field                         |
| 5351887970784238592                    | 457418232  | B8III     | 9.4641  | 9-10   | 2.1626     | -                                     |
| 5544723515521376000                    | 145338612  | B9IV      | 8.9543  | 7-8    | 4.8953     | <a href="#">Samus et al. 2003</a>     |
| 5759325125577015424                    | 919588     | B9V       | 9.3182  | 8      | 4.7913     | UCAC2 30191283 21" away               |
| 584063737770574976                     | 800147867  | DA        | 18.9288 | 8      | 3.1586     | -                                     |
| 5902486663443800448                    | 125080859  | A0III     | 9.5032  | 11     | 5.5032     | -                                     |
| <b>Primary eclipses only:</b>          |            |           |         |        |            |                                       |
| 5590218008142683520                    | 22641187   | B0V       | 15.7491 | 7      | 0.1018     | CV ( <a href="#">Ak et al. 2013</a> ) |
| 5864602303103277568                    | 320863824  | B1/2(III) | 9.9408  | 11     | 0.4452     | -                                     |
| <b>Eccentric orbits:</b>               |            |           |         |        |            |                                       |
| 2975118421398967424                    | 146472758  | A         | 13.2714 | 5      | 3.8133     | -                                     |
| 3834352875505630080                    | 842028390  | DA        | 18.7803 | 8      | 14.7223    | object 8" away                        |

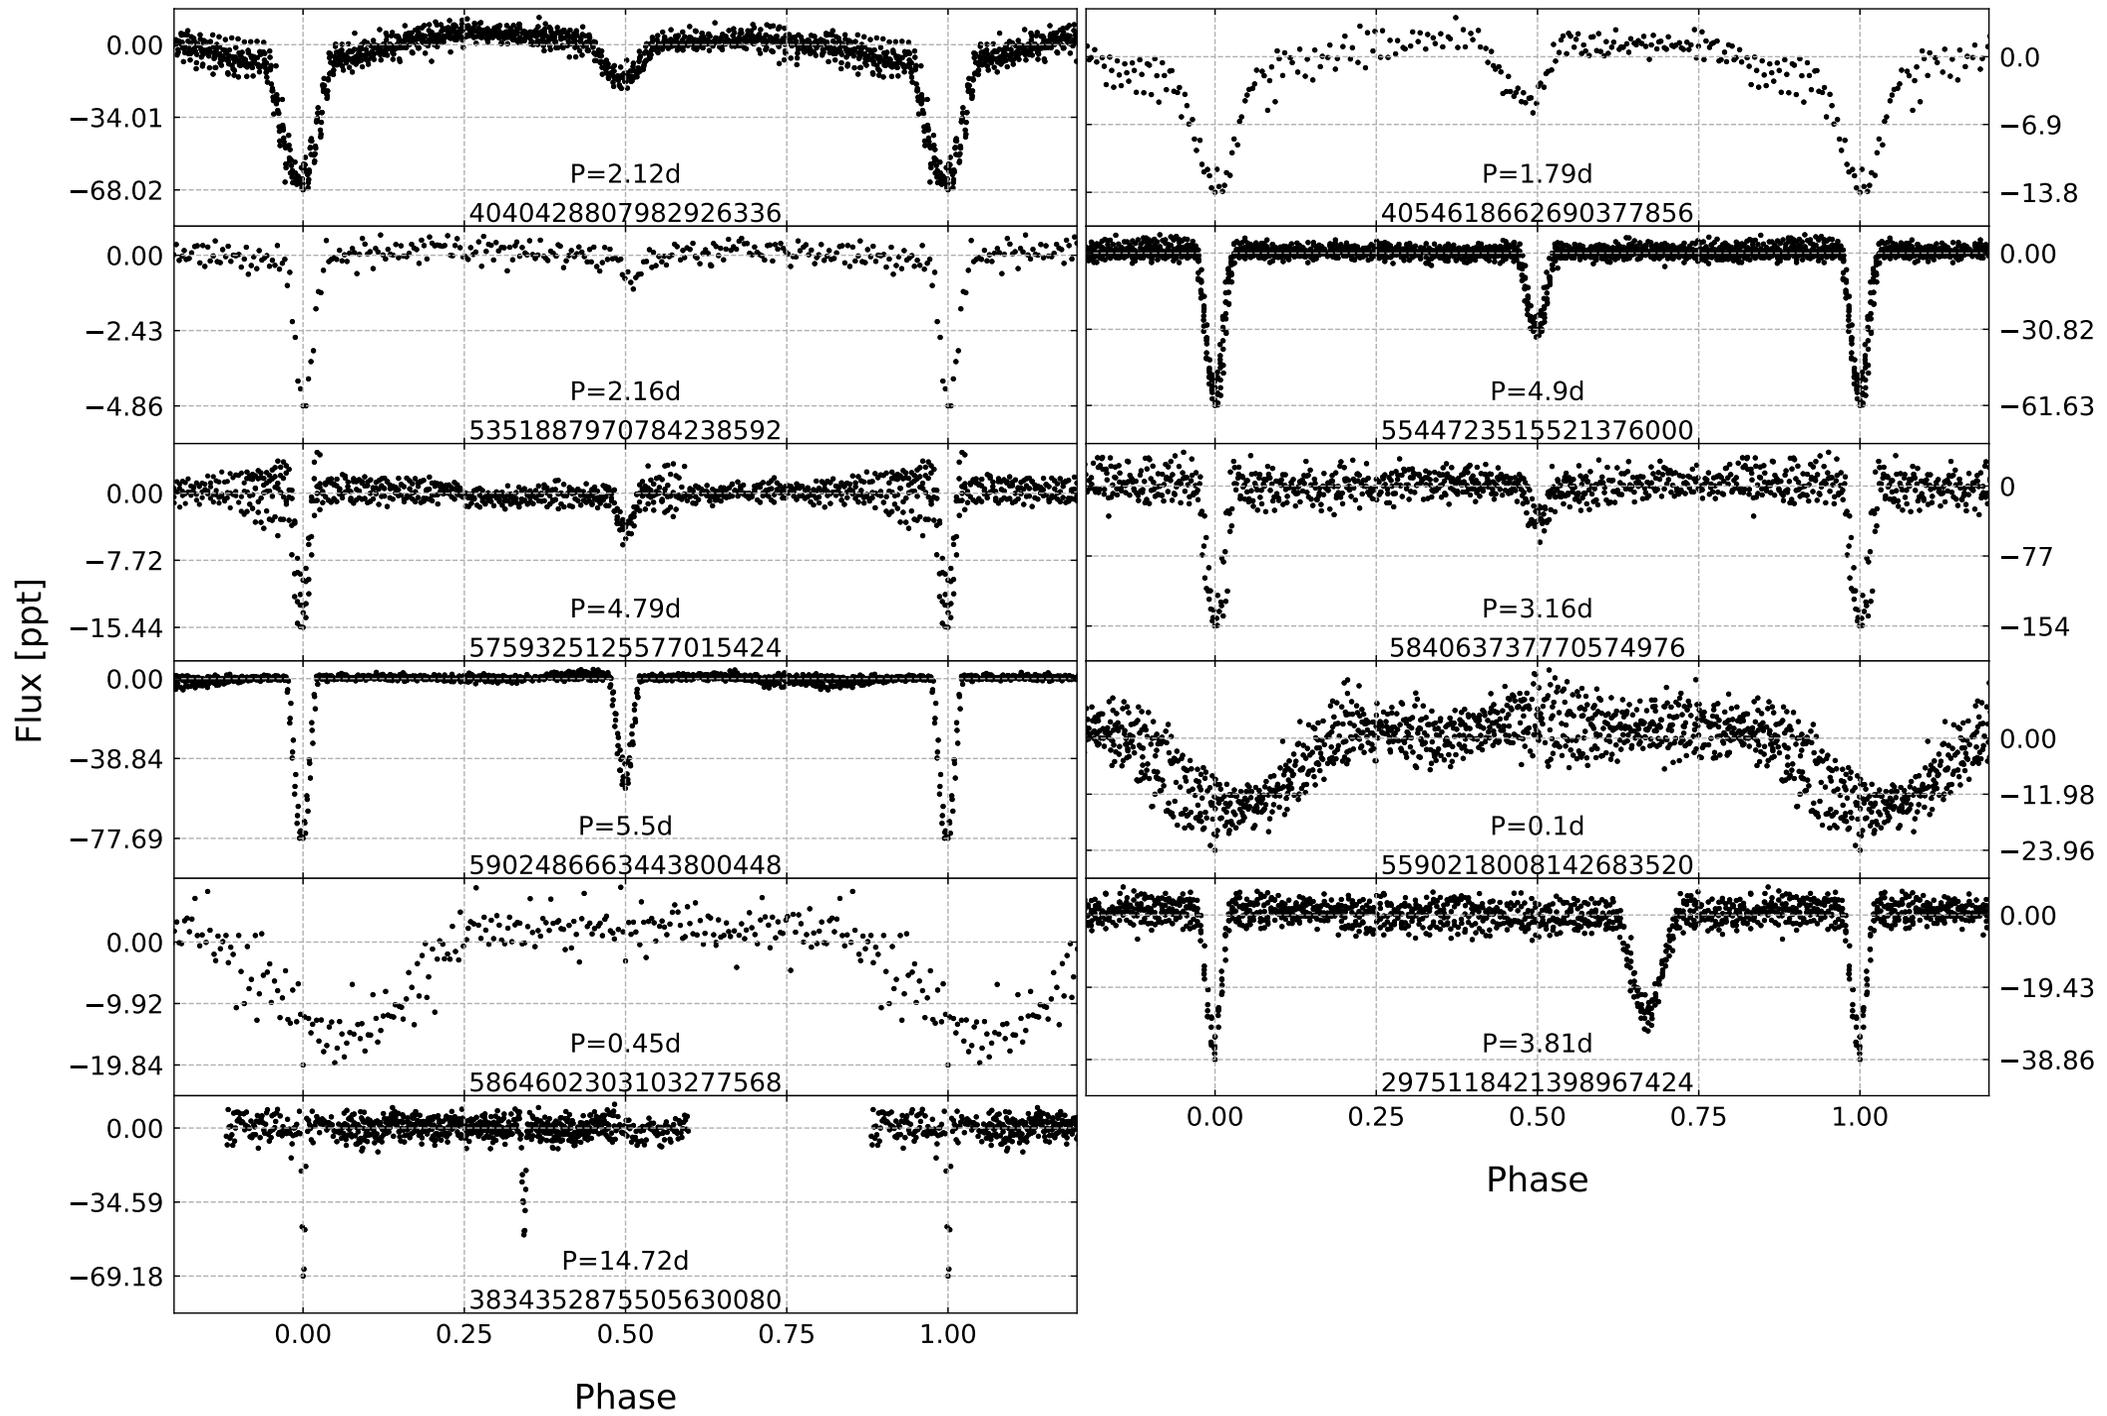

Supplement: Supplementary file 1 [file spec_eb.pdf]
