# Supplementary material for: A search for variable subdwarf B stars in TESS Full Frame Images -- I. Variable objects in the southern ecliptic hemisphere
Source: arXiv:2011.03465 ancillary file (2020-11-06)

**Basic information of 36 spectroscopically classified variables. The table is followed by amplitude spectra of these targets.**

| Gaia DR2            | TIC        | Spec Type | G mag   | Sector | Remarks                |
|---------------------|------------|-----------|---------|--------|------------------------|
| 2912264869258467200 | 37770142   | A0V       | 9.0304  | 6      | -                      |
| 2948419495935518848 | 148295706  | OB        | 11.2919 | 7      | -                      |
| 3052873581621063936 | 125200530  | A0V       | 8.2454  | 7      | -                      |
| 3305764520174154752 | 284729168  | B         | 16.4030 | 5      | -                      |
| 3344334627867111168 | 151473446  | B:        | 12.1872 | 6      | -                      |
| 3469365322037142016 | 170494530  | B2        | 13.0129 | 10     | -                      |
| 3477724290468772736 | 57793227   | B         | 15.8910 | 10     | -                      |
| 3480524609146540672 | 322809249  | B         | 12.5093 | 10     | -                      |
| 3490536212271814400 | 397419834  | B5        | 10.4823 | 10     | CD-25 8901 0.2" away   |
| 3491614283423744512 | 901474003  | B6        | 13.3266 | 10     | -                      |
| 3555477217298285312 | 391824371  | B7        | 13.3385 | 9      | -                      |
| 3753639444897348096 | 307936918  | A1        | 13.6254 | 9      | -                      |
| 4786097841386890496 | 161635091  | B         | 14.3731 | 4-5,6  | -                      |
| 4870606614334908928 | 686060362  | sdO       | 16.7833 | 4-5    | -                      |
| 4882954645311111424 | 686241564  | sdOHe     | 16.6324 | 4,5    | -                      |
| 4895712416167202176 | 44895938   | B3        | 14.5460 | 4-5    | -                      |
| 5329579463984075520 | 815576241  | A0        | 10.1893 | 8-9    | -                      |
| 5453052901782552704 | 49044042   | B6        | 11.1164 | 9      | -                      |
| 5700782320455378176 | 176304380  | B9IV/V    | 9.6313  | 7      | -                      |
| 578539413395848704  | 800042858  | DA+M      | 18.2978 | 8      | -                      |
| 5820064282494545280 | 1108525154 | B9III     | 13.7519 | 12     | -                      |
| 5825954366325225728 | 423426730  | B9V       | 8.1153  | 12     | TYC 9030-46-2 1" away  |
| 5864647692301841792 | 380846698  | A5/8      | 9.8842  | 11     | -                      |
| 5877234901498723840 | 404098422  | B3IV      | 6.3700  | 11-12  | HD 129092C 2" away     |
| 5884832114451618688 | 75708367   | B3/5V     | 8.1914  | 12     | TYC 8701-64-2 1" away  |
| 5926114786038289280 | 213207249  | B9/9.5V   | 8.8109  | 12     | -                      |
| 6106849625493901824 | 159197255  | OB+       | 12.5291 | 11     | -                      |
| 6137173602134028416 | 30989907   | OB+       | 11.8841 | 11     | -                      |
| 6155114264643246336 | 103778583  | B         | 11.6420 | 10     | -                      |
| 6409230097816994432 | 403284330  | B         | 13.1898 | 1      | object 21" away        |
| 6434081912466526080 | 382366857  | OB        | 11.4274 | 13     | -                      |
| 6442023272633436672 | 1922709746 | B         | 16.2533 | 13     | 2 objects within 42"   |
| 6485148764374844800 | 126658450  | B2He?     | 11.5218 | 1      | -                      |
| 6590537602435136768 | 89433335   | B3        | 13.4007 | 1      | -                      |
| 6630629472878877056 | 365660822  | OB+       | 12.2961 | 13     | -                      |
| 6706089368210943104 | 364952416  | A1/2V     | 7.9472  | 13     | TYC 8365-709-2 1" away |

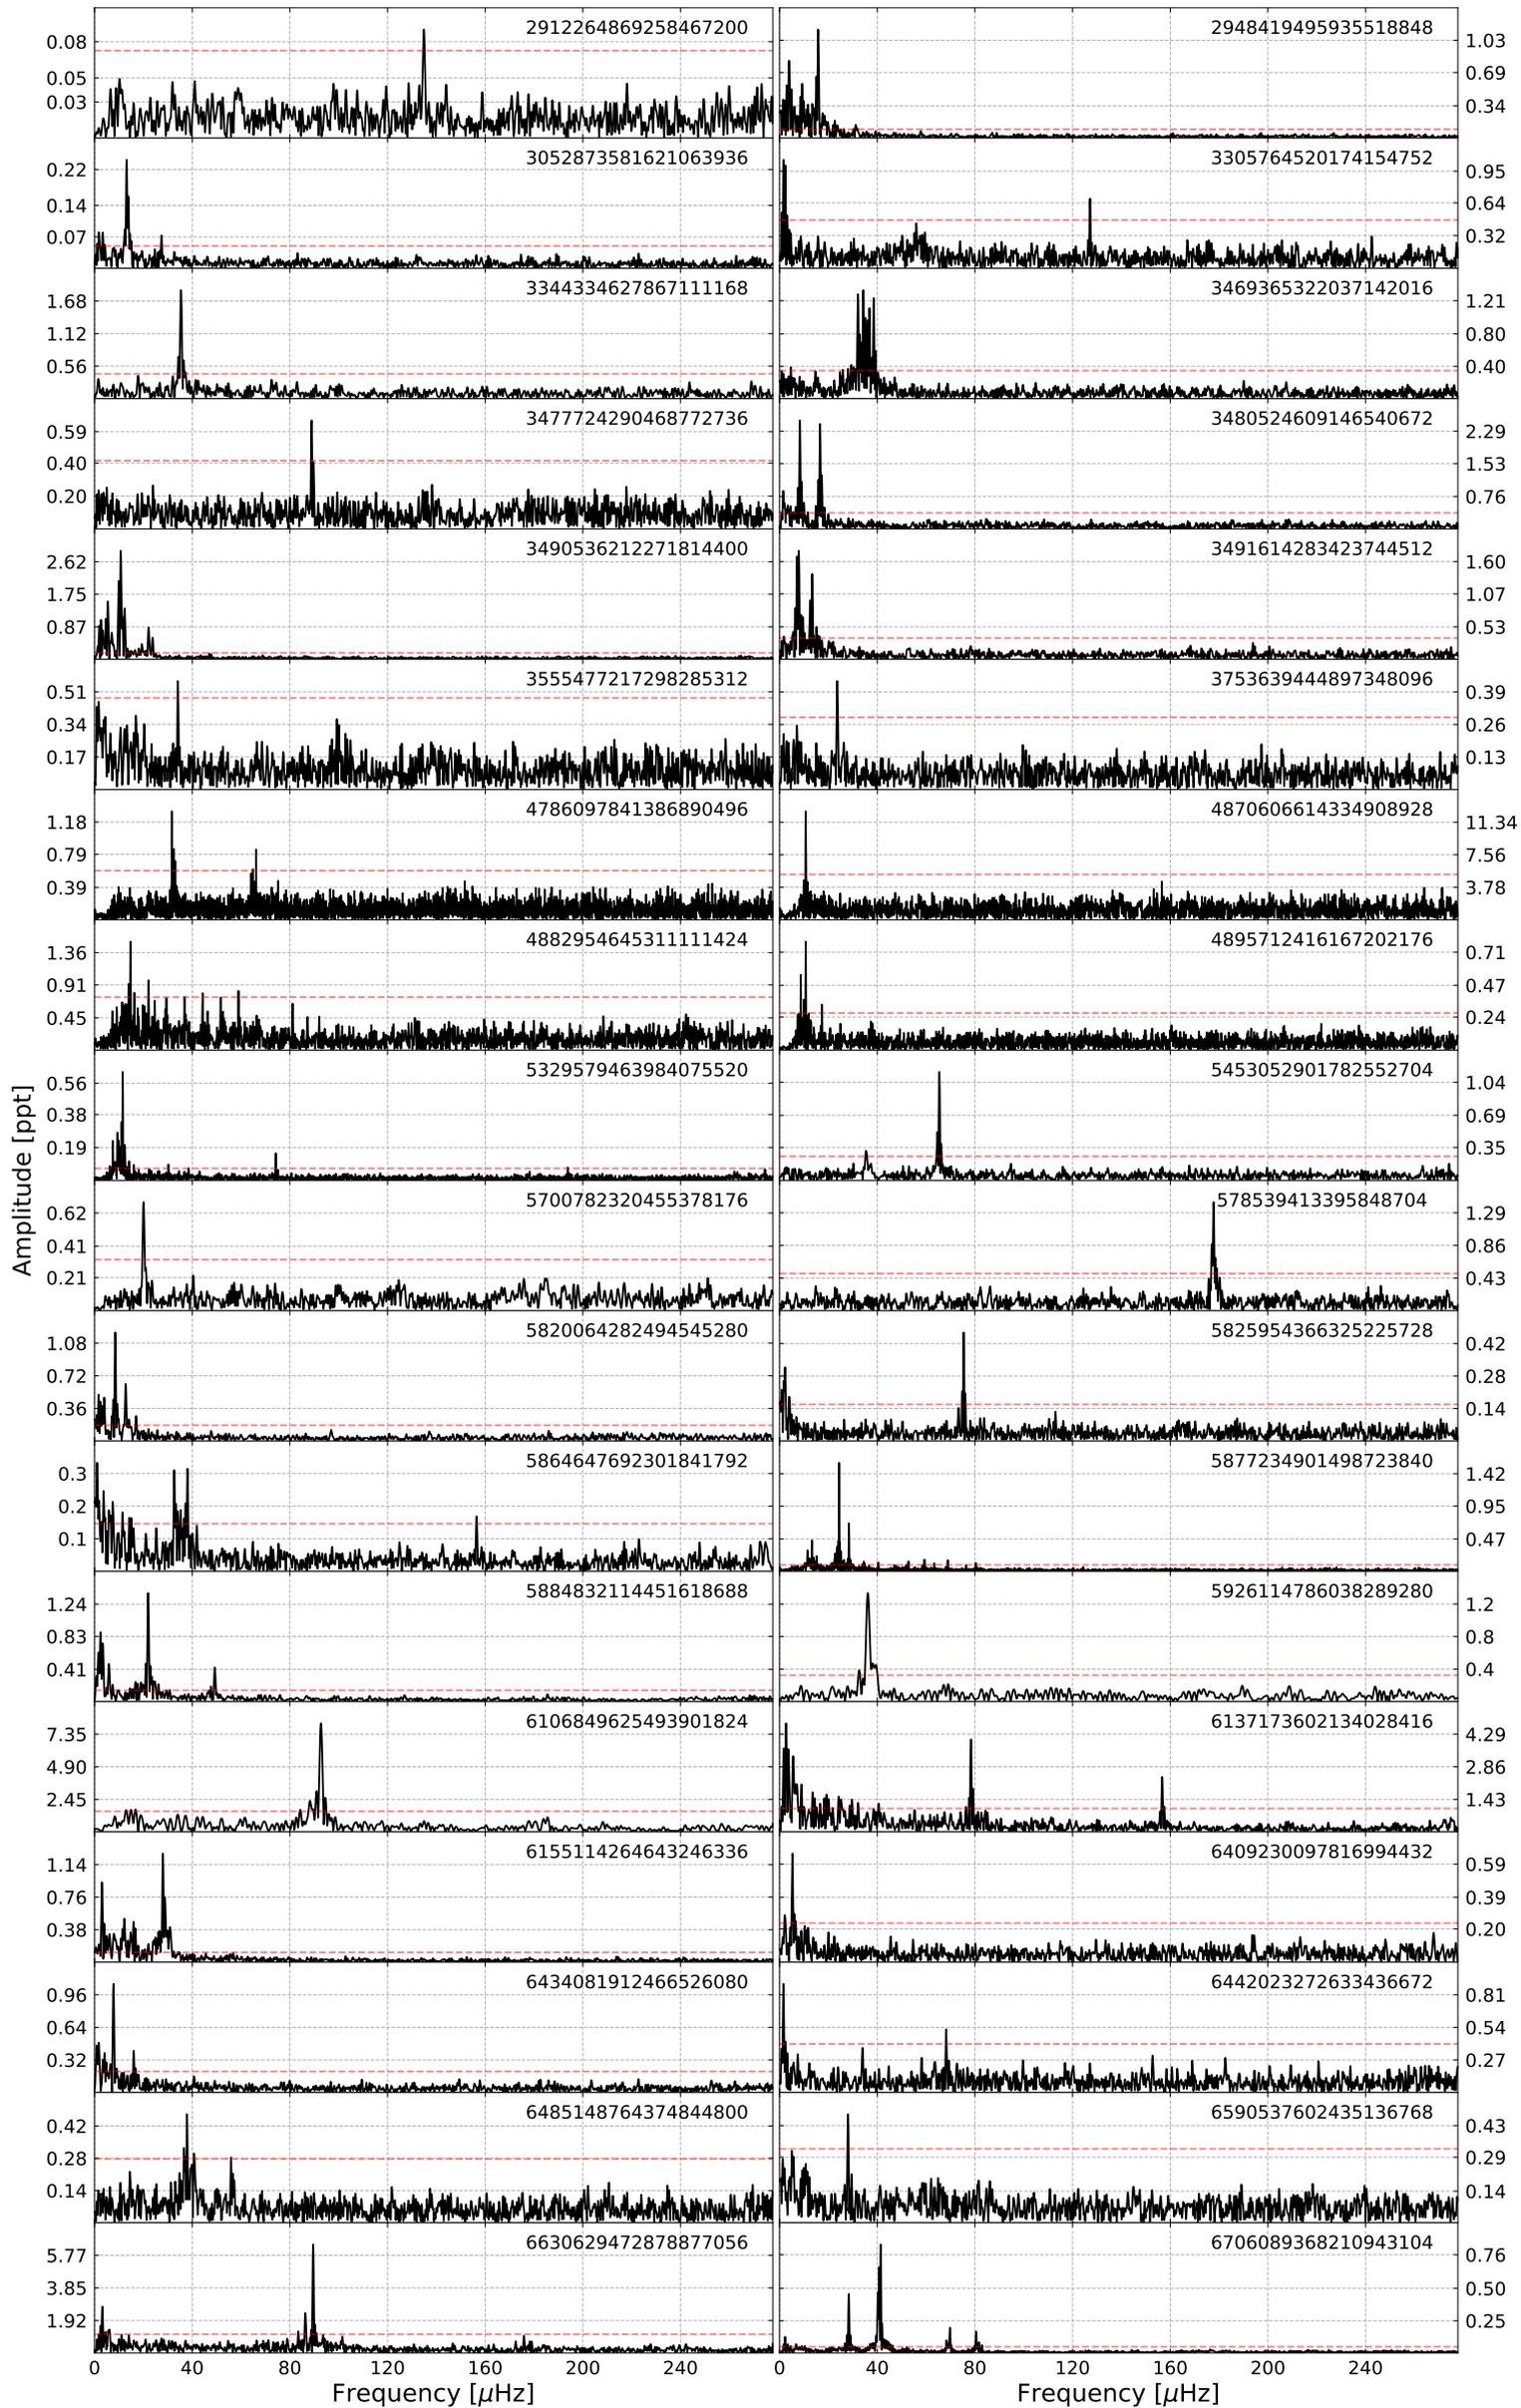

Supplement: Supplementary file 2 [file spec_ft.pdf]
