# Supplementary material for: A search for variable subdwarf B stars in TESS Full Frame Images -- I. Variable objects in the southern ecliptic hemisphere
Source: arXiv:2011.03465 ancillary file (2020-11-06)

Basic information of 15 spectroscopically classified variables. The table is followed by phased lightcurves of these targets.

| Gaia DR2                                      | TIC        | Spec Type  | G mag   | Sector | Period [d] | Remarks                              |
|-----------------------------------------------|------------|------------|---------|--------|------------|--------------------------------------|
| <b>Variables with one symmetric maximum:</b>  |            |            |         |        |            |                                      |
| 2382531303846872448                           | 12970429   | A0         | 13.8458 | 2      | 0.059      | -                                    |
| 3484255561335762560                           | 270373840  | B2V        | 10.3985 | 10     | 0.6759     | -                                    |
| 4686168482281917824                           | 184134822  | B0-5(III)e | 15.9332 | 1-2,13 | 0.8253     | -                                    |
| 4822681238943011840                           | 78015136   | B          | 13.1594 | 5-6    | 2.0625     | -                                    |
| 5362804330246457344                           | 120596335  | sdO        | 12.1774 | 10     | 0.3574     | <a href="#">Ratzloff et al. 2020</a> |
| 5641012078094779904                           | 829062665  | A0IV       | 8.0976  | 8      | 1.6344     | UCAC3 118-113569 22" away            |
| 5810017903018854784                           | 293896689  | OB-        | 10.5958 | 12-13  | 3.873      | <a href="#">Ratzloff et al. 2020</a> |
| 6066705249078471296                           | 253275342  | B8V        | 8.1019  | 11     | 0.4812     | TYC 8652-2102-2 1" away              |
| 6369440112037710592                           | 327727051  | B4e        | 11.3631 | 13     | 0.9279     | TYC 9461-747-1 47" away              |
| 6375470177401596416                           | 419571251  | B3         | 11.8572 | 13     | 2.463      | -                                    |
| 6818355106040261376                           | 25202305   | B6         | 12.0939 | 1      | 2.7991     | -                                    |
| <b>Variables with one asymmetric maximum:</b> |            |            |         |        |            |                                      |
| 6720095737595795200                           | 88985610   | A1V        | 8.8523  | 13     | 2.6584     | TYC 8358-1002-1 30" away             |
| <b>Variables with two maxima:</b>             |            |            |         |        |            |                                      |
| 4038633133701623168                           | 1559025737 | B8V        | 8.7413  | 13     | 2.026      | HD 165063 4" away                    |
| 6204768798167836032                           | 75647221   | OB-        | 11.5776 | 11     | 0.5561     | -                                    |
| 6799118570294811264                           | 212299724  | B5III      | 10.4408 | 1      | 1.8268     | 4 objects within 3.5'                |

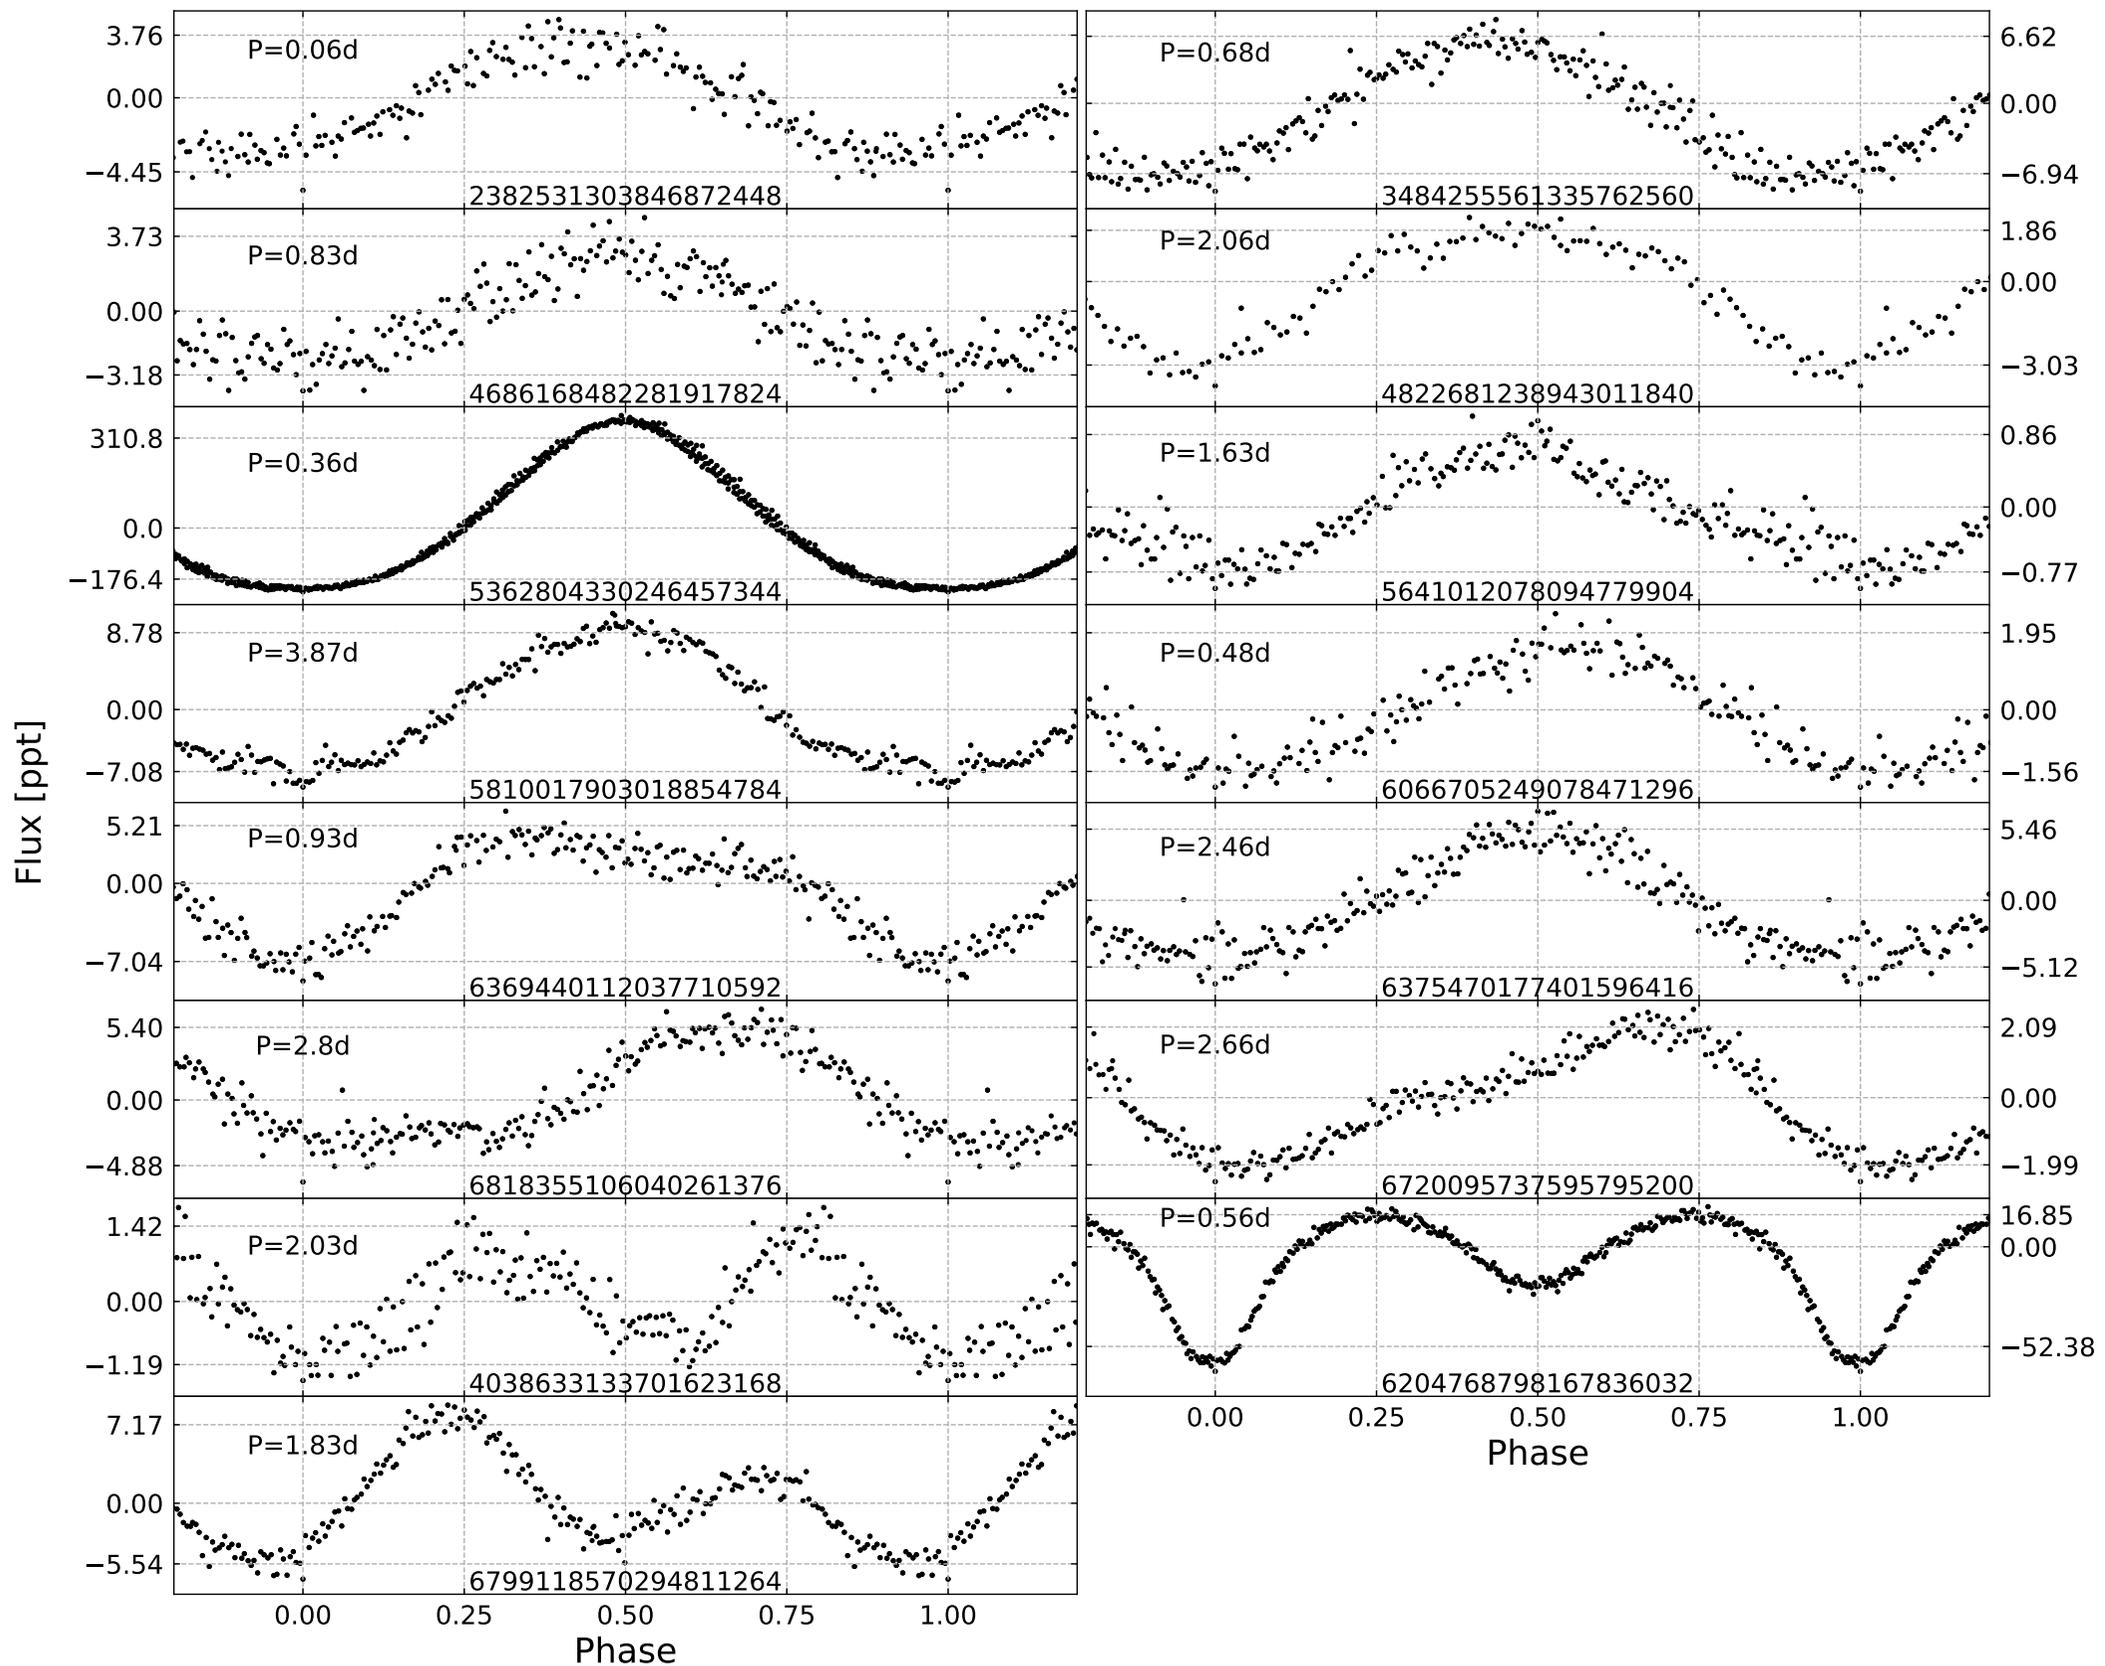

Supplement: Supplementary file 3 [file spec_phased.pdf]
