# Supplementary material for: A search for variable subdwarf B stars in TESS Full Frame Images -- I. Variable objects in the southern ecliptic hemisphere
Source: arXiv:2011.03465 ancillary file (2020-11-06)

**Basic information of 14 spectroscopically classified pulsators. The table is followed by amplitude spectra of these targets.**

| <b>Gaia DR2</b>     | <b>TIC</b> | <b>Spec Type</b> | <b>G mag</b> | <b>Sector</b> | <b>Remarks</b>                         |
|---------------------|------------|------------------|--------------|---------------|----------------------------------------|
| 2969201399574096128 | 708596809  | A0IV/V           | 11.3038      | 5-6           | -                                      |
| 3109409266919646976 | 168595004  | A5               | 10.7013      | 7             | -                                      |
| 3115125211261708032 | 293137161  | A0               | 11.0109      | 7             | -                                      |
| 3344114626761364224 | 437889214  | B5               | 10.0241      | 6             | -                                      |
| 3396397877830881792 | 247513086  | A0               | 8.1678       | 6             | -                                      |
| 4817132519153233792 | 77436693   | BHe              | 13.7017      | 4-5           | -                                      |
| 5090382015016433920 | 686449995  | A5mA5-F2         | 6.6339       | 4-5           | TYC 5889-321-2 1" away                 |
| 5326745919424790656 | 126486580  | A0V              | 9.1569       | 8-9           | TYC 8169-958-2 0.3" away               |
| 5429254969036524416 | 4595563    | A2/3(IV)         | 10.0846      | 8-9           | -                                      |
| 5524551806479093376 | 29796977   | A0               | 9.9794       | 8-9           | -                                      |
| 5796399012705196800 | 401975322  | B1III            | 10.2127      | 12            | CPD-72 1542B 4" away                   |
| 6534581776366266752 | 224284872  | A0               | 13.5498      | 2             | <a href="#">Holdsworth et al. 2014</a> |
| 654222239006166656  | 740003685  | DAO/sdOB         | 15.9301      | 7             | -                                      |
| 6702965728696663424 | 349351160  | A7               | 10.6141      | 13            | -                                      |

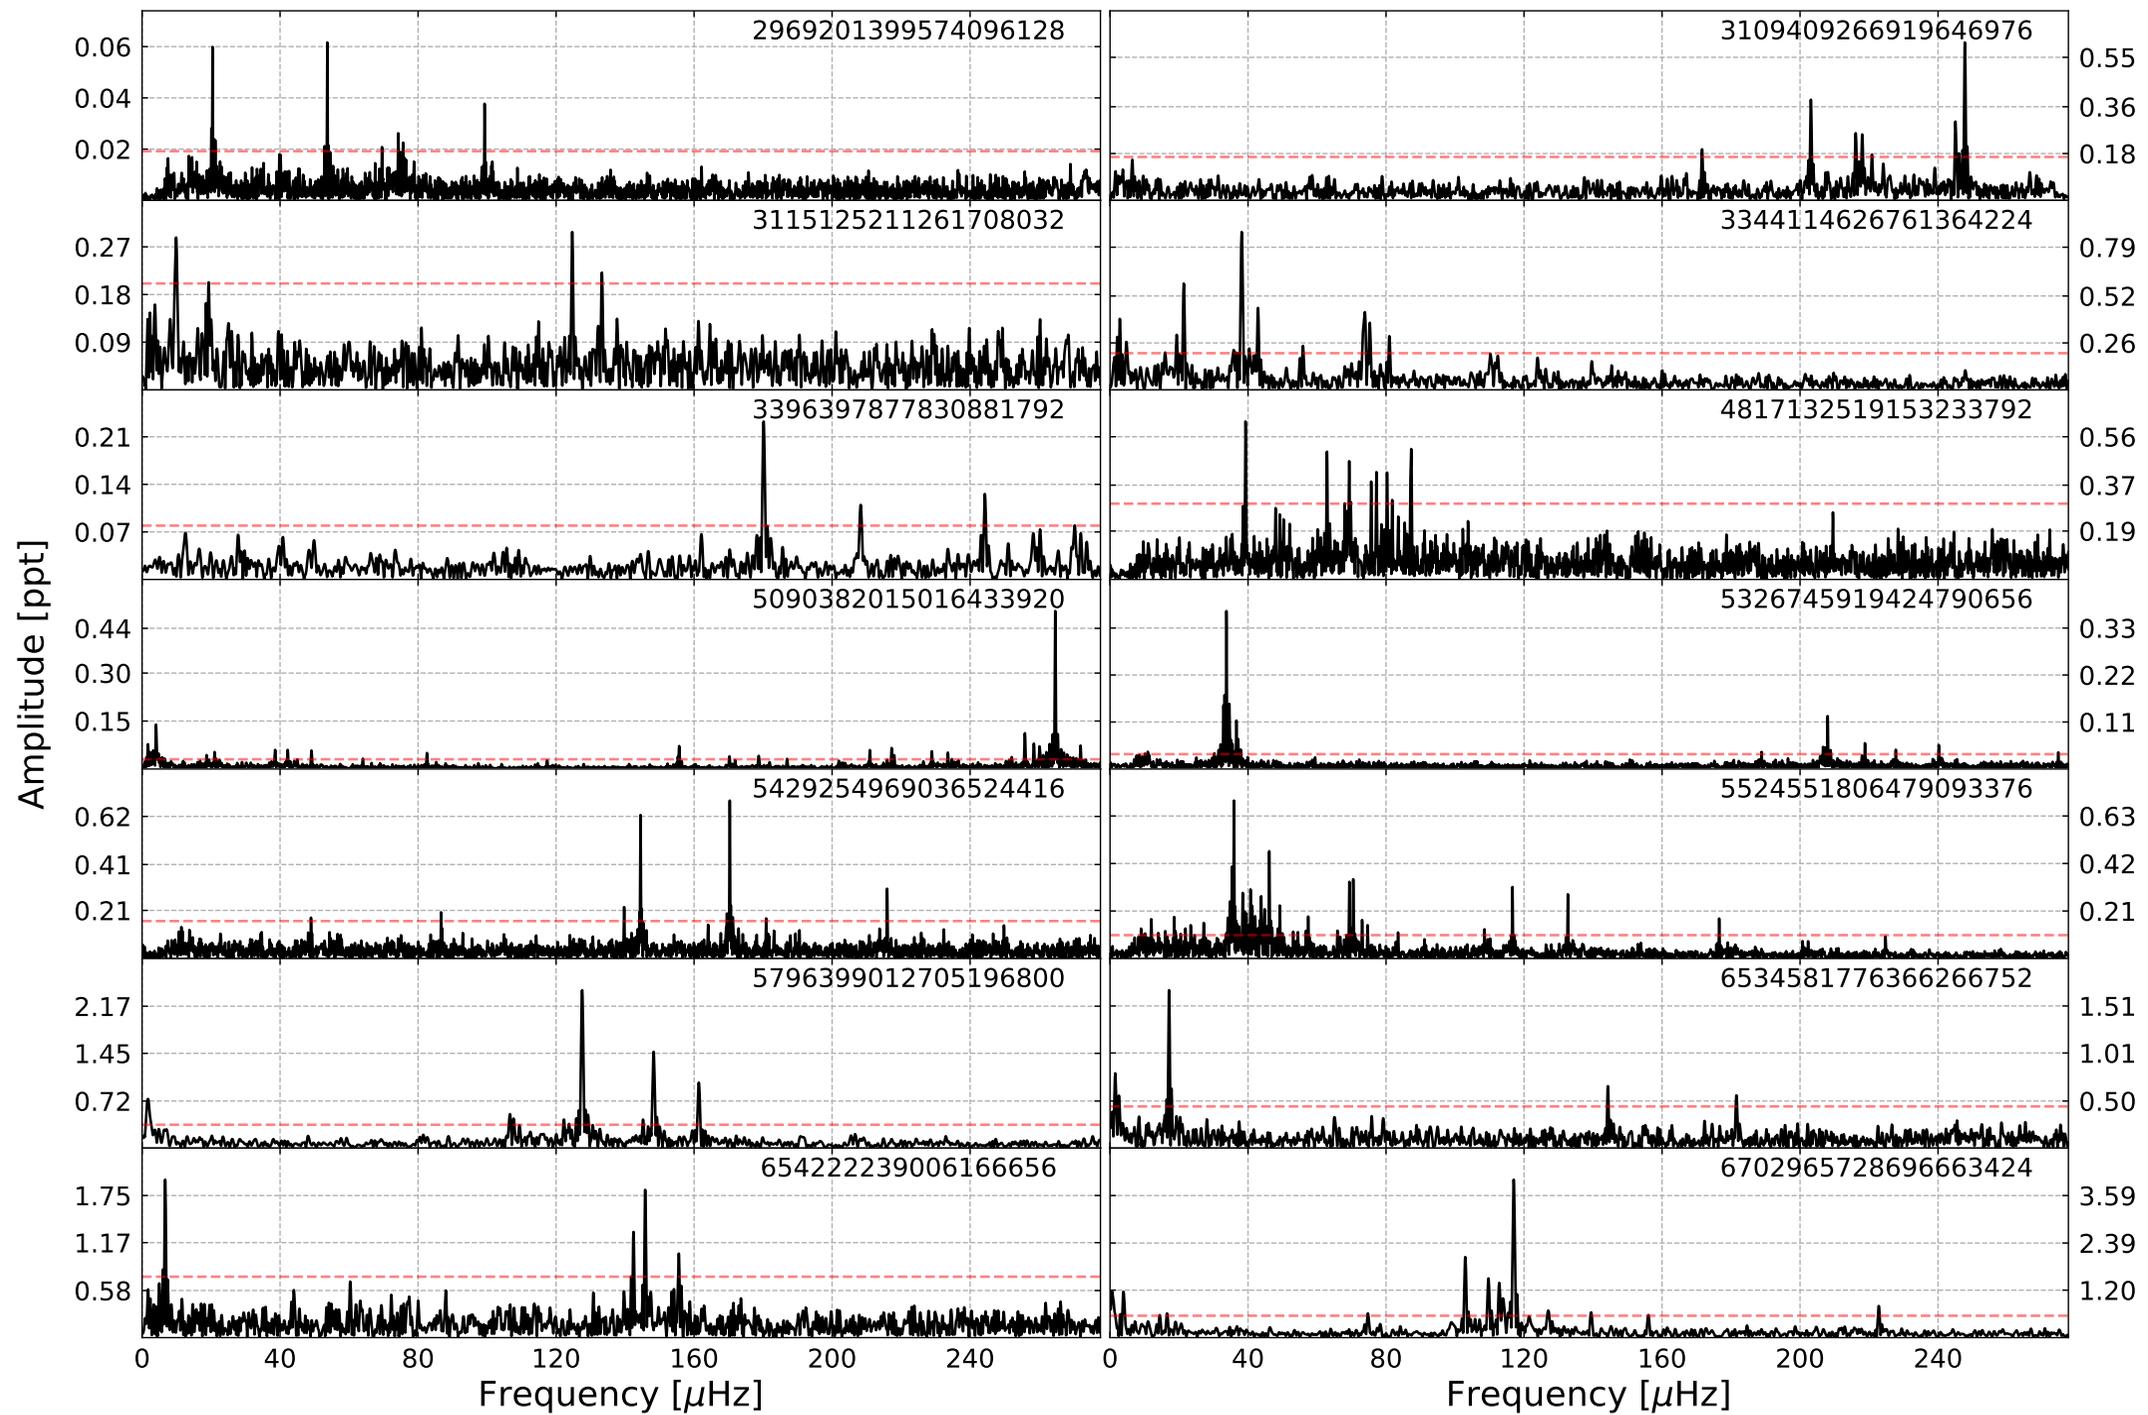

Supplement: Supplementary file 4 [file spec_pulsators.pdf]
