# Supplementary material for: A search for variable subdwarf B stars in TESS Full Frame Images -- I. Variable objects in the southern ecliptic hemisphere
Source: arXiv:2011.03465 ancillary file (2020-11-06)

Table 6 and Figure 10 continued...

**Basic information of 28 spectroscopically unclassified variables showing one asymmetric maximum. The table is followed by phased lightcurves of these targets.**

| Gaia DR2            | TIC        | G mag   | Sector | Period [d] | Remarks                              |
|---------------------|------------|---------|--------|------------|--------------------------------------|
| 2922539741007440768 | 79689537   | 16.7037 | 6-7    | 3.125      | crowded field                        |
| 2927154597462957056 | 48524451   | 14.4955 | 6-7    | 0.2488     | <a href="#">Skiff 1999</a>           |
| 2957940029686164352 | 708350288  | 18.1023 | 5-6    | 0.7407     | very crowded field                   |
| 3047774184120137088 | 752216365  | 18.5000 | 7      | 5.8824     | crowded field                        |
| 3786348167772858368 | 902790976  | 17.7064 | 9      | 0.6849     | -                                    |
| 4702811313050785280 | 39017348   | 16.4710 | 1-2    | 0.8065     | object 14" away                      |
| 5304690746979284480 | 809316750  | 18.4262 | 8-10   | 0.3788     | crowded field                        |
| 5383736493312165248 | 940928992  | 15.7916 | 10     | 1.7857     | CD-39 7118B 19" away                 |
| 5393973114069348096 | 941900430  | 17.4699 | 9      | 0.5348     | object 16" away                      |
| 5439868103801897600 | 873480537  | 16.6583 | 8-9    | 0.0873     | object 19" away                      |
| 5461053601219563520 | 71338192   | 10.9956 | 9      | 2.0408     | -                                    |
| 5579436712515286016 | 96520292   | 13.1680 | 6-7    | 1.2987     | -                                    |
| 5689491195023189248 | 296724066  | 14.3763 | 8      | 2.2727     | -                                    |
| 5719124334768705920 | 54275411   | 12.0252 | 7      | 1.5625     | -                                    |
| 5821920567383105664 | 1207491680 | 17.6124 | 12     | 0.4065     | crowded field                        |
| 5824470506633796480 | 1110873767 | 17.3381 | 12     | 3.4483     | crowded field                        |
| 5865963326711336832 | 325986533  | 13.1195 | 11     | 1.087      | -                                    |
| 5914259512380607872 | 174187648  | 14.1760 | 12     | 0.4717     | crowded field                        |
| 5917758433248059776 | 1511991718 | 18.7700 | 13     | 0.6238     | 2 bright objects within 21"          |
| 5945298691274098304 | 363483973  | 16.4243 | 13     | 0.4505     | 2 bright objects within 21"          |
| 5947381578621154432 | 363706224  | 11.8104 | 13     | 0.2247     | <a href="#">Ratzloff et al. 2020</a> |
| 5951113321119542528 | 217365202  | 13.3547 | 12     | 0.7929     | bright object 18" away               |
| 6039655274470700544 | 1172278318 | 17.1057 | 12     | 0.4878     | 2 bright objects within 21"          |
| 6118854333959388672 | 1054281677 | 18.9556 | 11     | 0.6897     | -                                    |
| 6724239453327875072 | 1698634750 | 17.3710 | 13     | 0.5102     | crowded field                        |
| 6733781534926708096 | 1705468240 | 18.2017 | 13     | 0.4587     | crowded field                        |
| 6734982648321929216 | 1707147184 | 16.6171 | 13     | 0.4405     | very crowded field                   |
| 6735459595828246400 | 1823921368 | 18.9920 | 13     | 0.525      | crowded field                        |

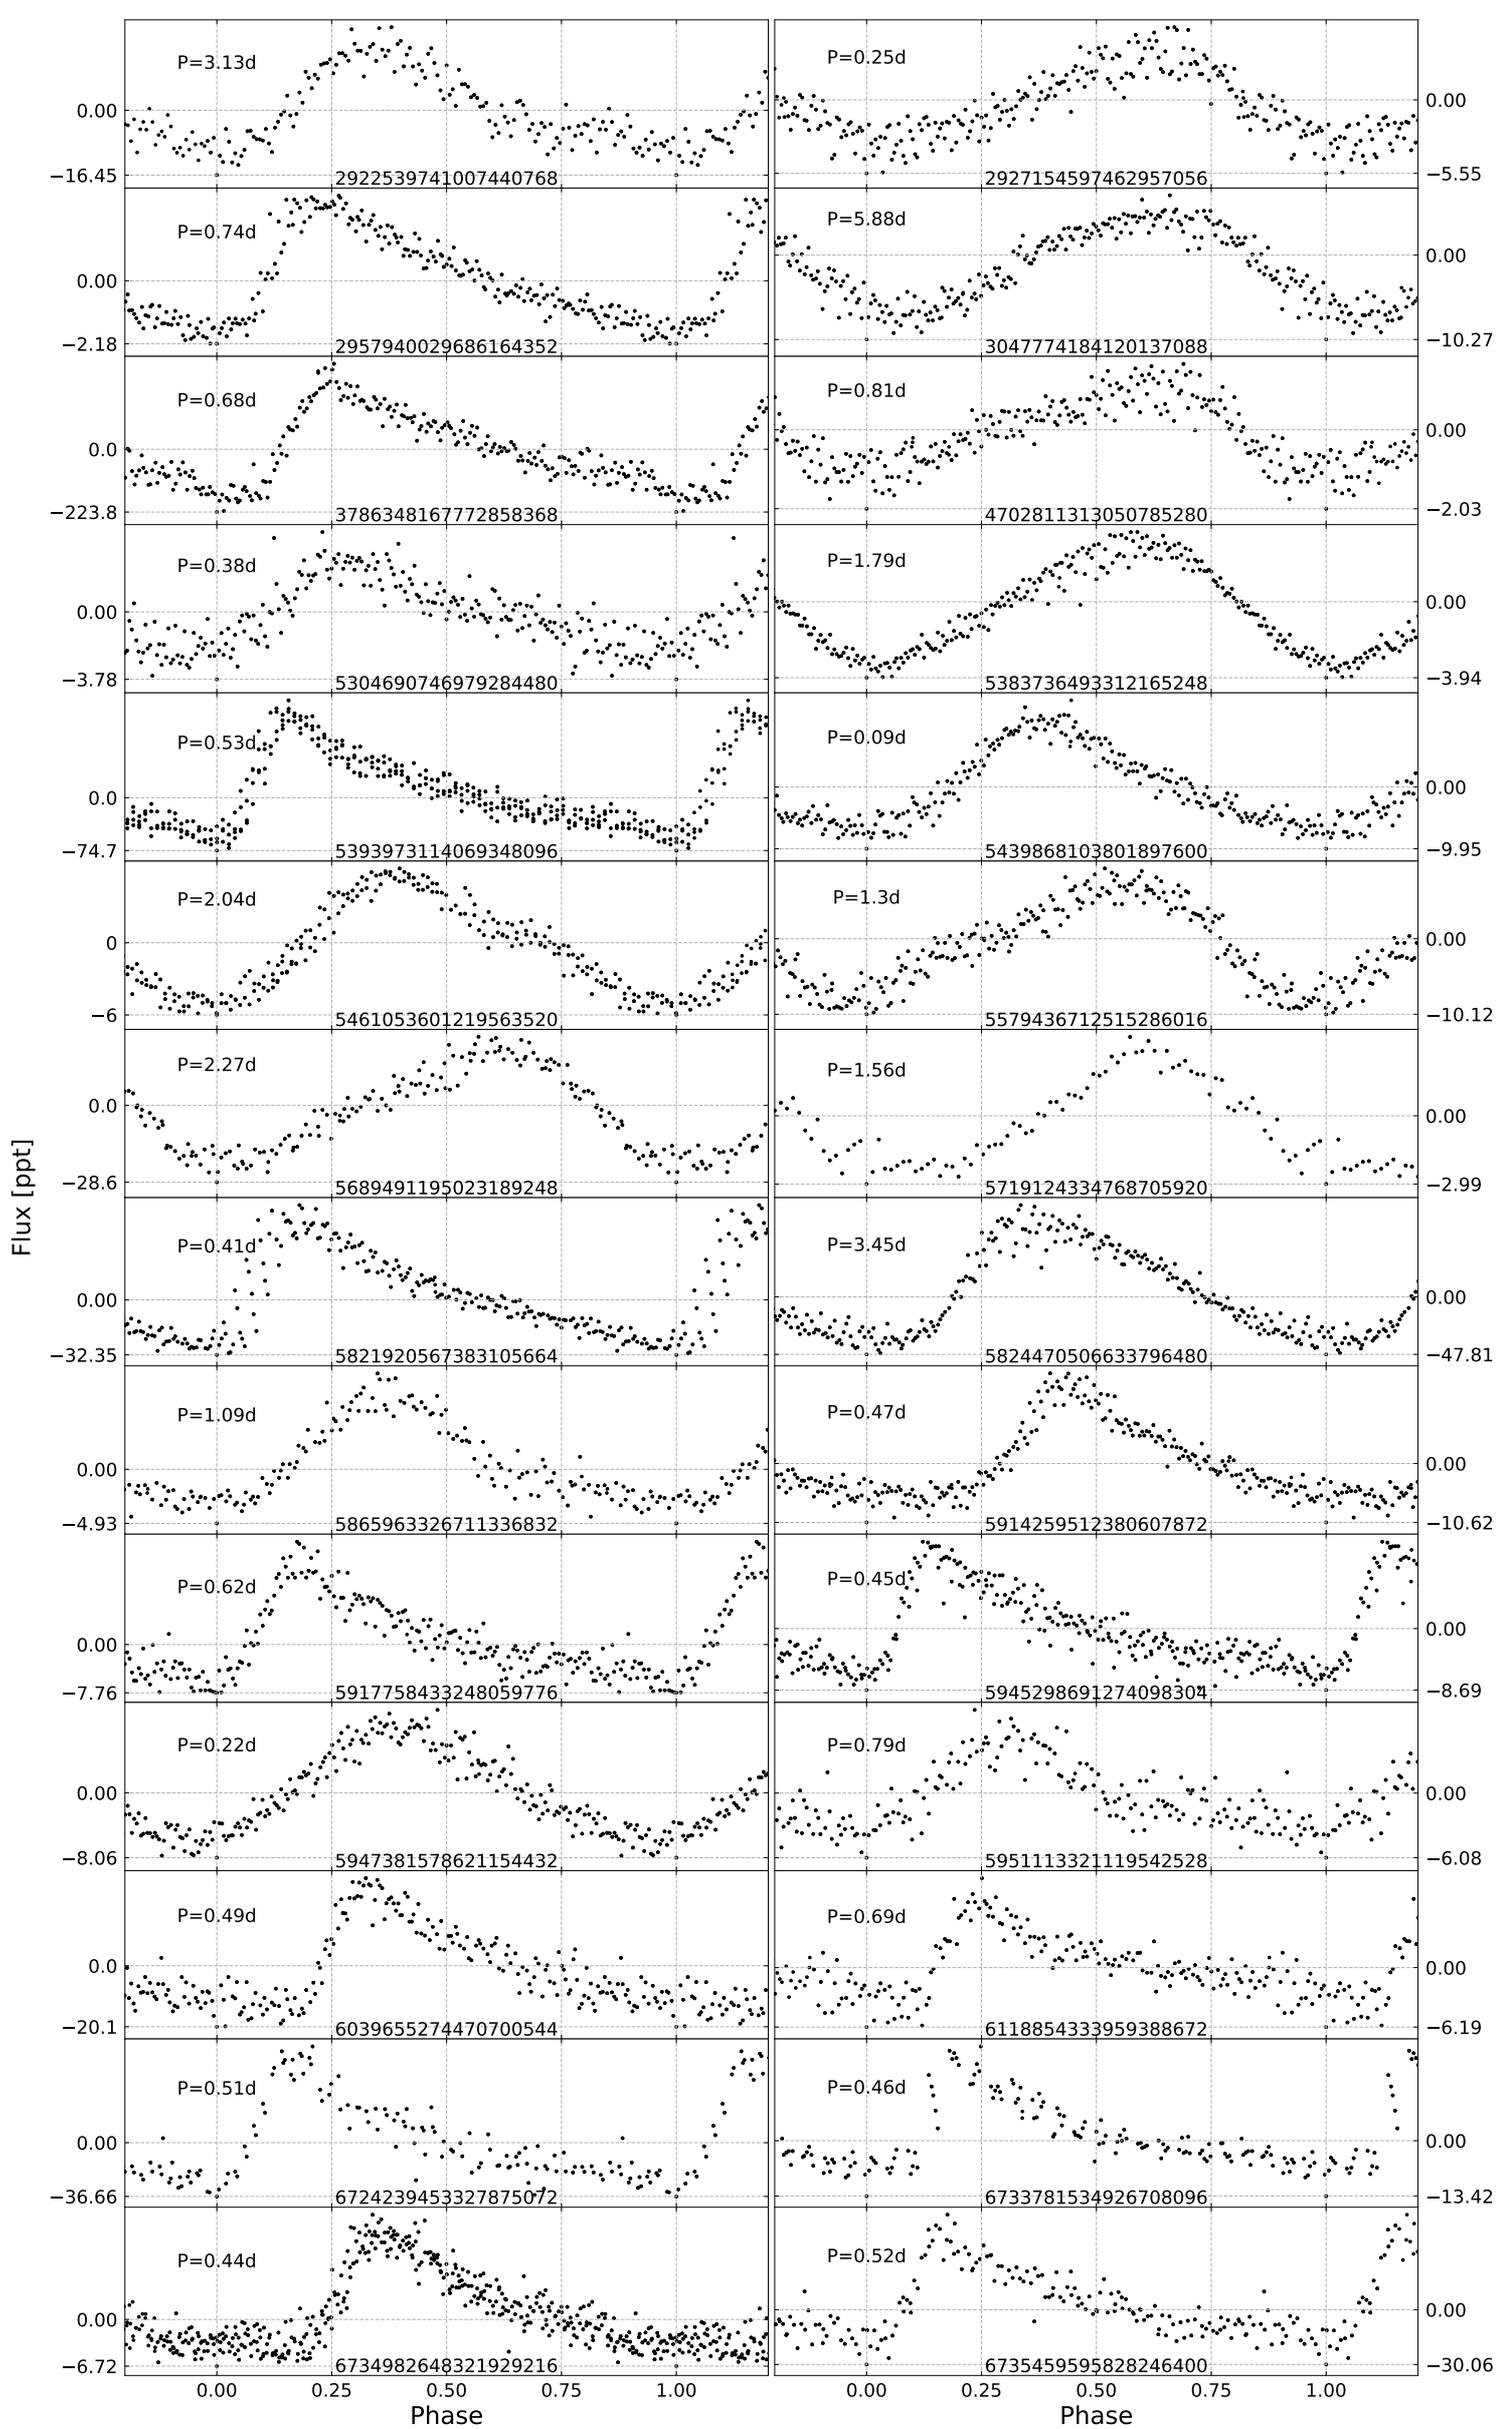

Supplement: Supplementary file 5 [file nospec_phased_1asymmetric.pdf]
