# Supplementary material for: A search for variable subdwarf B stars in TESS Full Frame Images -- I. Variable objects in the southern ecliptic hemisphere
Source: arXiv:2011.03465 ancillary file (2020-11-06)

Table 6 and Figure 10 continued...

**Basic information of 170 spectroscopically unclassified variables showing one symmetric maximum. The table is followed by phased lightcurves of these targets.**

| Gaia DR2            | TIC        | G mag   | Sector          | Period [d] | Remarks                                                              |
|---------------------|------------|---------|-----------------|------------|----------------------------------------------------------------------|
| 2896588449084891136 | 49547169   | 13.2752 | 6               | 0.3086     | -                                                                    |
| 2905822663130146688 | 31353391   | 14.0306 | 5-6             | 0.8929     | -                                                                    |
| 2909497952544966272 | 37118148   | 14.2848 | 6               | 0.2681     | object 22" away                                                      |
| 2924341084643425024 | 49774041   | 10.6884 | 6               | 2.439      | -                                                                    |
| 2936588029269162624 | 60348471   | 14.4922 | 6               | 2.439      | 2 objects within 12"                                                 |
| 2957941296696980608 | 708356594  | 17.8818 | 5-6             | 0.339      | very crowded field                                                   |
| 2993468995592753920 | 34264736   | 15.9326 | 6               | 0.1761     | -                                                                    |
| 2995717462506292736 | 317804295  | 15.9389 | 6               | 0.1706     | <a href="#">Drake et al. 2014</a>                                    |
| 3006362139517524608 | 709860036  | 18.6935 | 6               | 2.1277     | bright object 18" away                                               |
| 3010515995663287424 | 332831934  | 16.4133 | 6               | 1.0417     | <a href="#">Drake et al. 2014</a>                                    |
| 3026543267432558336 | 139785230  | 15.9418 | 7               | 0.0937     | -                                                                    |
| 3038538526969624192 | 170301183  | 12.2852 | 7               | 3.0303     | object 8" away                                                       |
| 3049609165952551680 | 125264225  | 11.1178 | 7               | 1.1494     | -                                                                    |
| 3052993703264602112 | 177514185  | 14.6115 | 7               | 0.2564     | bright object 7" away                                                |
| 3055532608748900864 | 64730323   | 14.7393 | 7               | 0.6024     | object 19.80" away                                                   |
| 3061898441775753216 | 65145461   | 15.5720 | 7               | 0.1163     | -                                                                    |
| 3069130101545218560 | 803407565  | 10.9765 | 7               | 2.5641     | HD 66715 2" away                                                     |
| 3083335826137398400 | 803870626  | 16.2499 | 7               | 0.2653     | 2 objects within 21"                                                 |
| 3136176770124825216 | 759533492  | 18.3739 | 7               | 0.431      | object 17" away                                                      |
| 3150707232898463616 | 468928859  | 15.6014 | 7               | 0.266      | candidate sdB ( <a href="#">Pérez-Fernández et al. 2016</a> )        |
| 3151064780336438656 | 271207314  | 14.2113 | 7               | 0.142      | CV ( <a href="#">Carter et al. 2013</a> )                            |
| 3151362095151274752 | 19026014   | 15.3668 | 7               | 0.5525     | -                                                                    |
| 3217698036836906624 | 11197405   | 15.2110 | 6               | 0.0755     | -                                                                    |
| 3239171705085395072 | 672588015  | 17.4300 | 5               | 3.125      | bright object 16" away                                               |
| 3341157696395192320 | 716209046  | 18.7224 | 6               | 0.1745     | bright object 16" away                                               |
| 3468413690428028288 | 951159803  | 18.5900 | 10              | 0.1414     | CRTS J122641.7-333204 ( <a href="#">Drake et al. 2017</a> ) 31" away |
| 3480090194676896384 | 901200174  | 18.6582 | 10              | 0.5435     | -                                                                    |
| 3532585694447087232 | 20446816   | 12.9149 | 9               | 1.0753     | object 9" away                                                       |
| 3573965638463072768 | 902378838  | 18.5374 | 9               | 1.3889     | -                                                                    |
| 4035348484483331584 | 1401293420 | 18.4414 | 13              | 0.1946     | crowded field                                                        |
| 4038372381956935680 | 1558161606 | 18.9364 | 13              | 0.5435     | very crowded field                                                   |
| 4038805177242745600 | 1559754008 | 18.9708 | 13              | 0.3745     | very crowded field                                                   |
| 4045364760494465024 | 1571918587 | 18.9518 | 13              | 2.439      | very crowded field                                                   |
| 4046774712424275200 | 1576915471 | 17.4836 | 13              | 0.2712     | very crowded field                                                   |
| 4716642550852732672 | 237907939  | 14.1971 | 1-2             | 0.1381     | -                                                                    |
| 4752367504705559936 | 146687440  | 14.6042 | 3-4             | 1.4925     | -                                                                    |
| 4756267369383483904 | 149599018  | 14.5860 | 1-13            | 5.8824     | -                                                                    |
| 4762428207898487168 | 685137498  | 18.4965 | 1-13            | 0.1346     | 3 objects within 21"                                                 |
| 4829447221183169024 | 206474978  | 15.9645 | 3-4             | 0.2155     | -                                                                    |
| 4909378967742431360 | 206564279  | 13.7836 | 2               | 1.4286     | object 14" away                                                      |
| 4927555166260455040 | 382416478  | 14.1480 | 2               | 0.7519     | -                                                                    |
| 5194902582490530560 | 804500973  | 18.0666 | 11-13           | 3.7037     | bright object 11" away                                               |
| 5196065251613078912 | 804549027  | 17.9476 | 11,13           | 0.1227     | object 17" away                                                      |
| 5199247646285490432 | 394563922  | 15.9390 | 11-12           | 0.1151     | object 16" away                                                      |
| 5201664480218395136 | 842747184  | 18.1610 | 11-13           | 1.3889     | object 19" away                                                      |
| 5213207393804130816 | 271888015  | 13.0316 | 1,3-4,6-7,10-13 | 0.8146     | -                                                                    |
| 5214328517707616128 | 271642755  | 13.5606 | 1-4,6-13        | 2.2222     | -                                                                    |
| 5231883973199654400 | 398791871  | 11.8203 | 10,11           | 1.1236     | -                                                                    |
| 5232515157294643712 | 844059251  | 18.7848 | 10              | 0.1845     | HD 91441 37" away                                                    |
| 5239154184595202048 | 844338903  | 18.2947 | 10-11           | 0.7407     | crowded field                                                        |
| 5239571311849267200 | 465456367  | 14.4587 | 10-11           | 1.8519     | crowded field                                                        |

|                     |           |         |               |        |                                                               |
|---------------------|-----------|---------|---------------|--------|---------------------------------------------------------------|
| 5242975056226807296 | 372815862 | 13.0191 | 10-11         | 1.2346 | object 23" away                                               |
| 5243482686998229376 | 371016851 | 14.3668 | 10-11         | 0.2415 | object 5" away                                                |
| 5244874526978221824 | 845251687 | 18.8808 | 10-11         | 0.5348 | 4 bright objects within 21"                                   |
| 5246146180897092608 | 845838164 | 17.6428 | 10-11         | 0.3106 | 2 objects within 21"                                          |
| 5249910741223769728 | 846930961 | 17.5118 | 9-11          | 2.0833 | HD 84865 17" away                                             |
| 5251560902025244416 | 377658867 | 15.2404 | 10            | 0.2132 | crowded field                                                 |
| 5266468802206471296 | 167250176 | 14.2593 | 1-4,6-13      | 0.1595 | -                                                             |
| 5270373786471521024 | 306505851 | 16.0345 | 1-13          | 0.1706 | -                                                             |
| 5291112774796009600 | 765677577 | 17.7893 | 4,7-10        | 0.1605 | -                                                             |
| 5293139655760876544 | 765773357 | 17.6631 | 1-4,6-13      | 3.4483 | bright object 13" away                                        |
| 5296462581763471104 | 356837752 | 16.2050 | 9-11          | 0.2639 | crowded field                                                 |
| 5296549340102210688 | 806872820 | 18.0098 | 9-10,11       | 3.8462 | -                                                             |
| 5298070003345815680 | 807215500 | 16.7830 | 9-11          | 0.1873 | object 19" away                                               |
| 5322521183433578752 | 388622589 | 10.8971 | 8-9           | 0.8475 | object nearby                                                 |
| 5341595751704487680 | 300685376 | 14.4953 | 10-11         | 1.9608 | crowded field                                                 |
| 5349904589251539456 | 82591181  | 13.0985 | 10            | 2.3256 | -                                                             |
| 5355588720798713728 | 862023654 | 16.6682 | 9-10          | 0.3663 | crowded field                                                 |
| 5355946268217174656 | 463006021 | 14.2694 | 9-10          | 1.2821 | crowded field                                                 |
| 5361576454936897664 | 937597821 | 18.5775 | 10            | 0.1724 | 3 objects within 21"                                          |
| 5363099308598820096 | 937974717 | 18.9485 | 9-10          | 0.2273 | 2 bright objects within 31"                                   |
| 5369091410756158080 | 400919731 | 13.9875 | 10            | 0.1447 | object 13" away                                               |
| 5371061903087037696 | 94246301  | 11.9477 | 10            | 4.1667 | -                                                             |
| 5388590356113794816 | 941437058 | 18.0723 | 10            | 0.2766 | -                                                             |
| 5390464817279368448 | 29917475  | 16.3367 | 9-10          | 0.3135 | bright object 19" away                                        |
| 5391620507080621824 | 158196468 | 12.9433 | 9-10          | 3.5714 | -                                                             |
| 5393463597805768320 | 158223878 | 12.0003 | 9,10          | 1.4493 | <a href="#">Ratzloff et al. 2020</a> ; TYC 7728-550-1 4" away |
| 5407683822210499072 | 867459631 | 18.9775 | 9-10          | 1.087  | TYC 8187-1501-1 14" away                                      |
| 5448344724273336064 | 71674519  | 14.4205 | 9             | 1.5152 | -                                                             |
| 5457161703718981504 | 942878246 | 18.5302 | 9             | 0.1479 | bright object 25" away                                        |
| 5477101965563632000 | 737151632 | 18.6176 | 1-7,9-13      | 1.6949 | 2 bright objects within 21"                                   |
| 5477508583007863936 | 149973540 | 13.4981 | 1-5,7-8,10-12 | 1.1364 | -                                                             |
| 5497677749426668800 | 238069203 | 14.1752 | 2,6-9,12      | 0.1555 | -                                                             |
| 5502168150617145216 | 238019887 | 15.2373 | 6-8           | 0.7692 | -                                                             |
| 5520454369017441664 | 818833960 | 18.7248 | 7-8           | 0.6369 | crowded field                                                 |
| 5526271511387514880 | 83081722  | 16.4120 | 8-9           | 0.1658 | -                                                             |
| 5546533513520296192 | 146117756 | 13.9041 | 7-8           | 0.1048 | crowded field                                                 |
| 5552604814865254400 | 170100070 | 15.3404 | 6-8           | 0.3165 | -                                                             |
| 5560208483233550720 | 770973891 | 18.7206 | 7             | 0.3484 | bright object 14" away                                        |
| 5576826952945841408 | 148044670 | 15.5495 | 6,7           | 0.3096 | -                                                             |
| 5584309675031744512 | 52388210  | 15.2471 | 6-7           | 0.3831 | -                                                             |
| 5591407473561155328 | 113929655 | 10.4655 | 7-8           | 0.6788 | -                                                             |
| 5611820525418596608 | 108121382 | 16.2622 | 7             | 0.207  | 3 objects within 21"                                          |
| 5615708084989439488 | 415143942 | 15.1695 | 7             | 0.1114 | -                                                             |
| 5627260280004729472 | 17460375  | 13.4378 | 8             | 0.1318 | object 15" away                                               |
| 5647085093133918720 | 196417751 | 11.8622 | 8             | 1.6393 | -                                                             |
| 5693570688108267648 | 831888569 | 18.4239 | 7-8           | 2.3256 | 6 objects within 21"                                          |
| 5696368773398103296 | 832623391 | 18.2993 | 7-8           | 0.4608 | -                                                             |
| 5697870946801360512 | 833025831 | 16.8982 | 7-8           | 0.0985 | 3 bright objects within 21"                                   |
| 5698379200347454208 | 833137917 | 18.6064 | 7-8           | 0.2597 | 5 objects within 21"                                          |
| 5709579959659083008 | 834573650 | 17.6760 | 8             | 0.1631 | object 29" away                                               |
| 5709912046530451840 | 405300501 | 15.3423 | 8             | 1.3699 | object 21" away                                               |
| 5715265255110912128 | 140674813 | 9.9703  | 7             | 3.8462 | -                                                             |
| 5716391812157166336 | 415224879 | 13.5069 | 7             | 0.2151 | 3 objects within 21"                                          |
| 5753841281270433536 | 51431668  | 15.2848 | 8             | 0.0889 | -                                                             |
| 5768566765625082112 | 384295509 | 14.0080 | 12,13         | 0.9009 | -                                                             |

|                     |            |         |       |        |                                                             |
|---------------------|------------|---------|-------|--------|-------------------------------------------------------------|
| 5785766490440028160 | 418757007  | 15.5599 | 12    | 0.1376 | 2 objects within 20"                                        |
| 5790175845607430656 | 396256097  | 16.9061 | 11-12 | 0.3717 | 2 objects within 20"                                        |
| 5796024319747525504 | 1106127339 | 18.2319 | 12    | 2.6316 | 2 objects within 21"                                        |
| 5802848777968872832 | 1309947558 | 18.2533 | 12,13 | 0.1422 | 2 objects within 21"                                        |
| 5804243753280956672 | 1309967972 | 18.8271 | 12,13 | 4.3478 | 3 bright objects within 21"                                 |
| 5809162246755246720 | 1206329315 | 18.3769 | 12    | 2.2727 | HD 149239 15" away                                          |
| 5810573710448599680 | 294196248  | 12.9580 | 12-13 | 1.2658 | -                                                           |
| 5810658029245818240 | 1509377483 | 15.5522 | 12-13 | 1.6667 | -                                                           |
| 5816413422869352448 | 1311566852 | 17.6044 | 12    | 0.1905 | object 13" away                                             |
| 5832749206423000832 | 1212998545 | 18.0591 | 12    | 0.4115 | 4 bright objects within 21"                                 |
| 5856360741911875840 | 448006966  | 16.7977 | 11    | 0.1175 | crowded field                                               |
| 5917085051098353152 | 1315252102 | 18.3548 | 12    | 0.2688 | 2 objects within 21"                                        |
| 5921549652415561856 | 1513801292 | 18.3068 | 12    | 1.9608 | crowded field                                               |
| 5929155867700733056 | 170432227  | 15.2404 | 12    | 0.2755 | crowded field                                               |
| 5946889718944314880 | 1517742678 | 18.7443 | 12    | 0.2985 | crowded field                                               |
| 5947682054521782400 | 1518444947 | 18.9835 | 13    | 0.8403 | 4 bright objects within 21"                                 |
| 5947917934120939264 | 1518643967 | 18.7456 | 13    | 1.6667 | 5 objects within 21"                                        |
| 5949607883502930560 | 1521051042 | 17.5739 | 12    | 0.3165 | crowded field                                               |
| 5949903476020736640 | 1521545612 | 17.5323 | 12    | 0.1629 | very crowded field                                          |
| 5951695443759022976 | 1523004908 | 18.6995 | 12    | 0.7874 | very crowded field                                          |
| 5951799313240078080 | 1523231725 | 18.5604 | 12    | 1.25   | crowded field                                               |
| 6003468079048102400 | 1167947965 | 18.1410 | 11    | 0.1681 | 2 objects within 21"                                        |
| 6005939265801702272 | 1168863300 | 17.8273 | 11    | 0.1608 | 3 objects within 21"                                        |
| 6057220728665468416 | 253184319  | 15.3899 | 11    | 0.4854 | 4 bright objects within 21"                                 |
| 6069641872841587200 | 1047202529 | 18.1091 | 11    | 1.2346 | -                                                           |
| 6085079806361861888 | 994074308  | 18.8981 | 11    | 0.4348 | 2 bright objects within 7"                                  |
| 6096267234097192320 | 242463073  | 12.1152 | 11    | 1.9231 | object 22" away                                             |
| 6098441797519559552 | 1172688066 | 18.9734 | 11    | 0.1852 | 3 objects within 21"                                        |
| 6104664243055570560 | 159259371  | 15.9112 | 11    | 0.152  | object 17.70" away                                          |
| 6132361177176695680 | 996245434  | 17.0499 | 10    | 0.1773 | CRTS J124318.8-453428 ( <a href="#">Drake et al. 2017</a> ) |
| 6148834236479971712 | 21641328   | 13.9621 | 10    | 1.0989 | -                                                           |
| 6155138767433459840 | 103831994  | 12.2167 | 10    | 1.1765 | <a href="#">Ratzloff et al. 2020</a>                        |
| 6157729113749149056 | 130924318  | 13.8970 | 10    | 0.5236 | -                                                           |
| 6159105255630163456 | 131236578  | 15.1397 | 10    | 0.2525 | CRTS J124541.3-335521 ( <a href="#">Drake et al. 2017</a> ) |
| 6359368722966483840 | 276796039  | 14.0759 | 12,13 | 4.7619 | -                                                           |
| 6381776422045939584 | 2054761216 | 18.9755 | 1,13  | 1.6393 | -                                                           |
| 6431145460504666752 | 1688544000 | 17.7551 | 12,13 | 5.5556 | -                                                           |
| 6461831833600743936 | 316788032  | 14.7836 | 1     | 1.0989 | -                                                           |
| 6562425082977942272 | 2027302068 | 17.0781 | 1     | 0.1645 | -                                                           |
| 6576260585683860736 | 147146907  | 15.3112 | 1     | 0.1441 | CV ( <a href="#">Kilkenny et al. 2015</a> )                 |
| 6629592225394313216 | 411918964  | 13.8330 | 13    | 0.1832 | -                                                           |
| 6636107617762820864 | 1816807538 | 17.9150 | 13    | 0.2053 | object 15" away                                             |
| 6657826477106032256 | 6665844    | 13.8368 | 13    | 1.4286 | object 14" away                                             |
| 6659367339573565312 | 1923720827 | 17.8642 | 13    | 0.4202 | 3 objects within 21"                                        |
| 6662709786201498240 | 1818609250 | 18.7813 | 13    | 0.2174 | 3 objects within 21"                                        |
| 6706393731068755840 | 1693385914 | 17.9470 | 13    | 2.0408 | crowded field                                               |
| 6707425171762916608 | 1693952468 | 18.9096 | 13    | 0.1305 | 2 bright objects within 21"                                 |
| 6709739098282201472 | 1694913243 | 17.6759 | 13    | 0.3521 | -                                                           |
| 6712934171688784256 | 1819863744 | 18.8697 | 13    | 0.8772 | bright object 20" away                                      |
| 6718384656985946112 | 1821060671 | 18.3488 | 13    | 1.4493 | 4 objects within 21"                                        |
| 6719608933120159744 | 1695222843 | 18.0591 | 13    | 1.0638 | crowded field                                               |
| 6721077154808040832 | 1696401635 | 18.6672 | 13    | 0.1684 | crowded field                                               |
| 6724206712797091456 | 1698589712 | 17.2689 | 13    | 0.2849 | very crowded field                                          |
| 6724526120927993600 | 1698985611 | 18.4472 | 13    | 0.4785 | crowded field                                               |
| 6727643648730503040 | 1703278418 | 18.2010 | 13    | 0.1783 | crowded field                                               |

|                     |            |         |    |        |                                                                    |
|---------------------|------------|---------|----|--------|--------------------------------------------------------------------|
| 6729391970973866752 | 1821836358 | 18.1346 | 13 | 0.3745 | Gaia DR2 6729391975273949184 ( <a href="#">Brown et al. 2018</a> ) |
| 6733034004471841664 | 1704918722 | 18.4647 | 13 | 0.3356 | 6 bright objects within 21"                                        |
| 6734105474265563136 | 1705799658 | 18.8796 | 13 | 0.3774 | crowded field                                                      |
| 6734417873003845888 | 1706301214 | 18.1017 | 13 | 0.2165 | very crowded field                                                 |
| 6742873224773448960 | 1925740295 | 18.3469 | 13 | 3.7037 | 2 objects within 21"                                               |
| 6743398202922849664 | 1825788527 | 18.5304 | 13 | 0.1506 | 4 objects within 21"                                               |
| 6760001859308263808 | 1827654125 | 18.4395 | 13 | 0.2309 | 6 objects within 21"                                               |
| 6761309114219270144 | 1828793177 | 18.2610 | 13 | 0.274  | Gaia DR2 6761309114226077952 5" away                               |
| 6794666712135593344 | 1992439824 | 18.1095 | 1  | 0.1484 | -                                                                  |

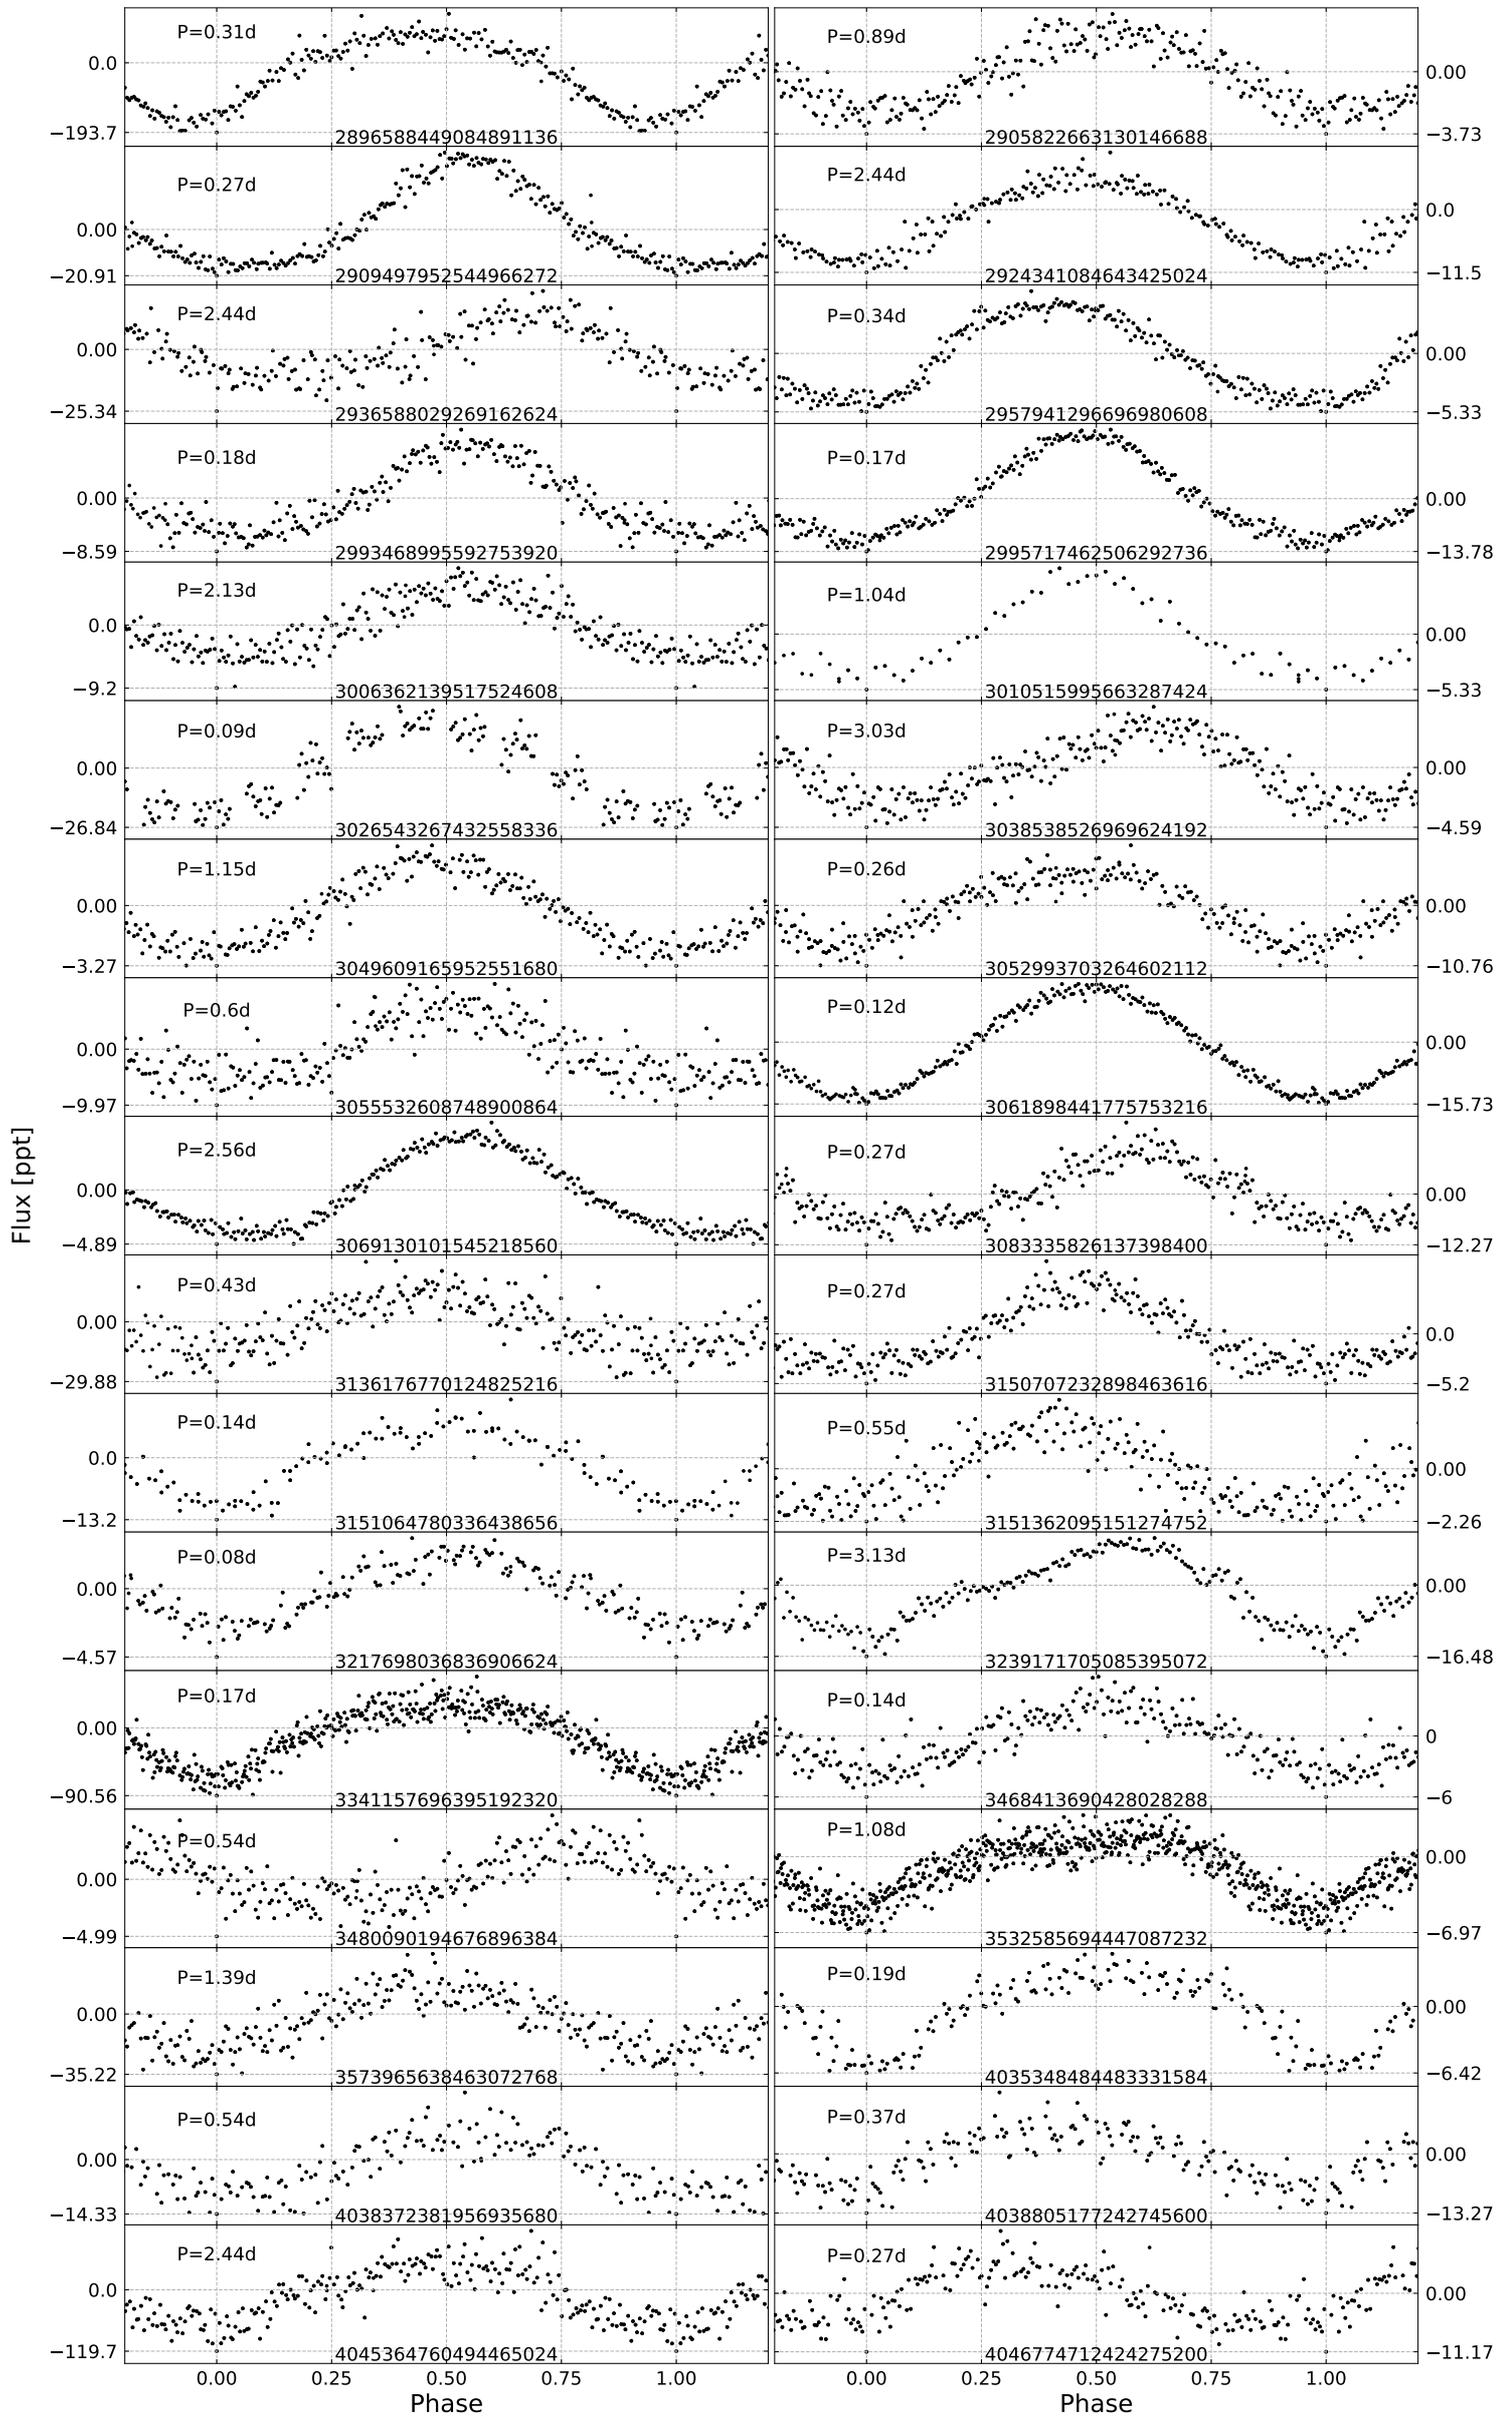

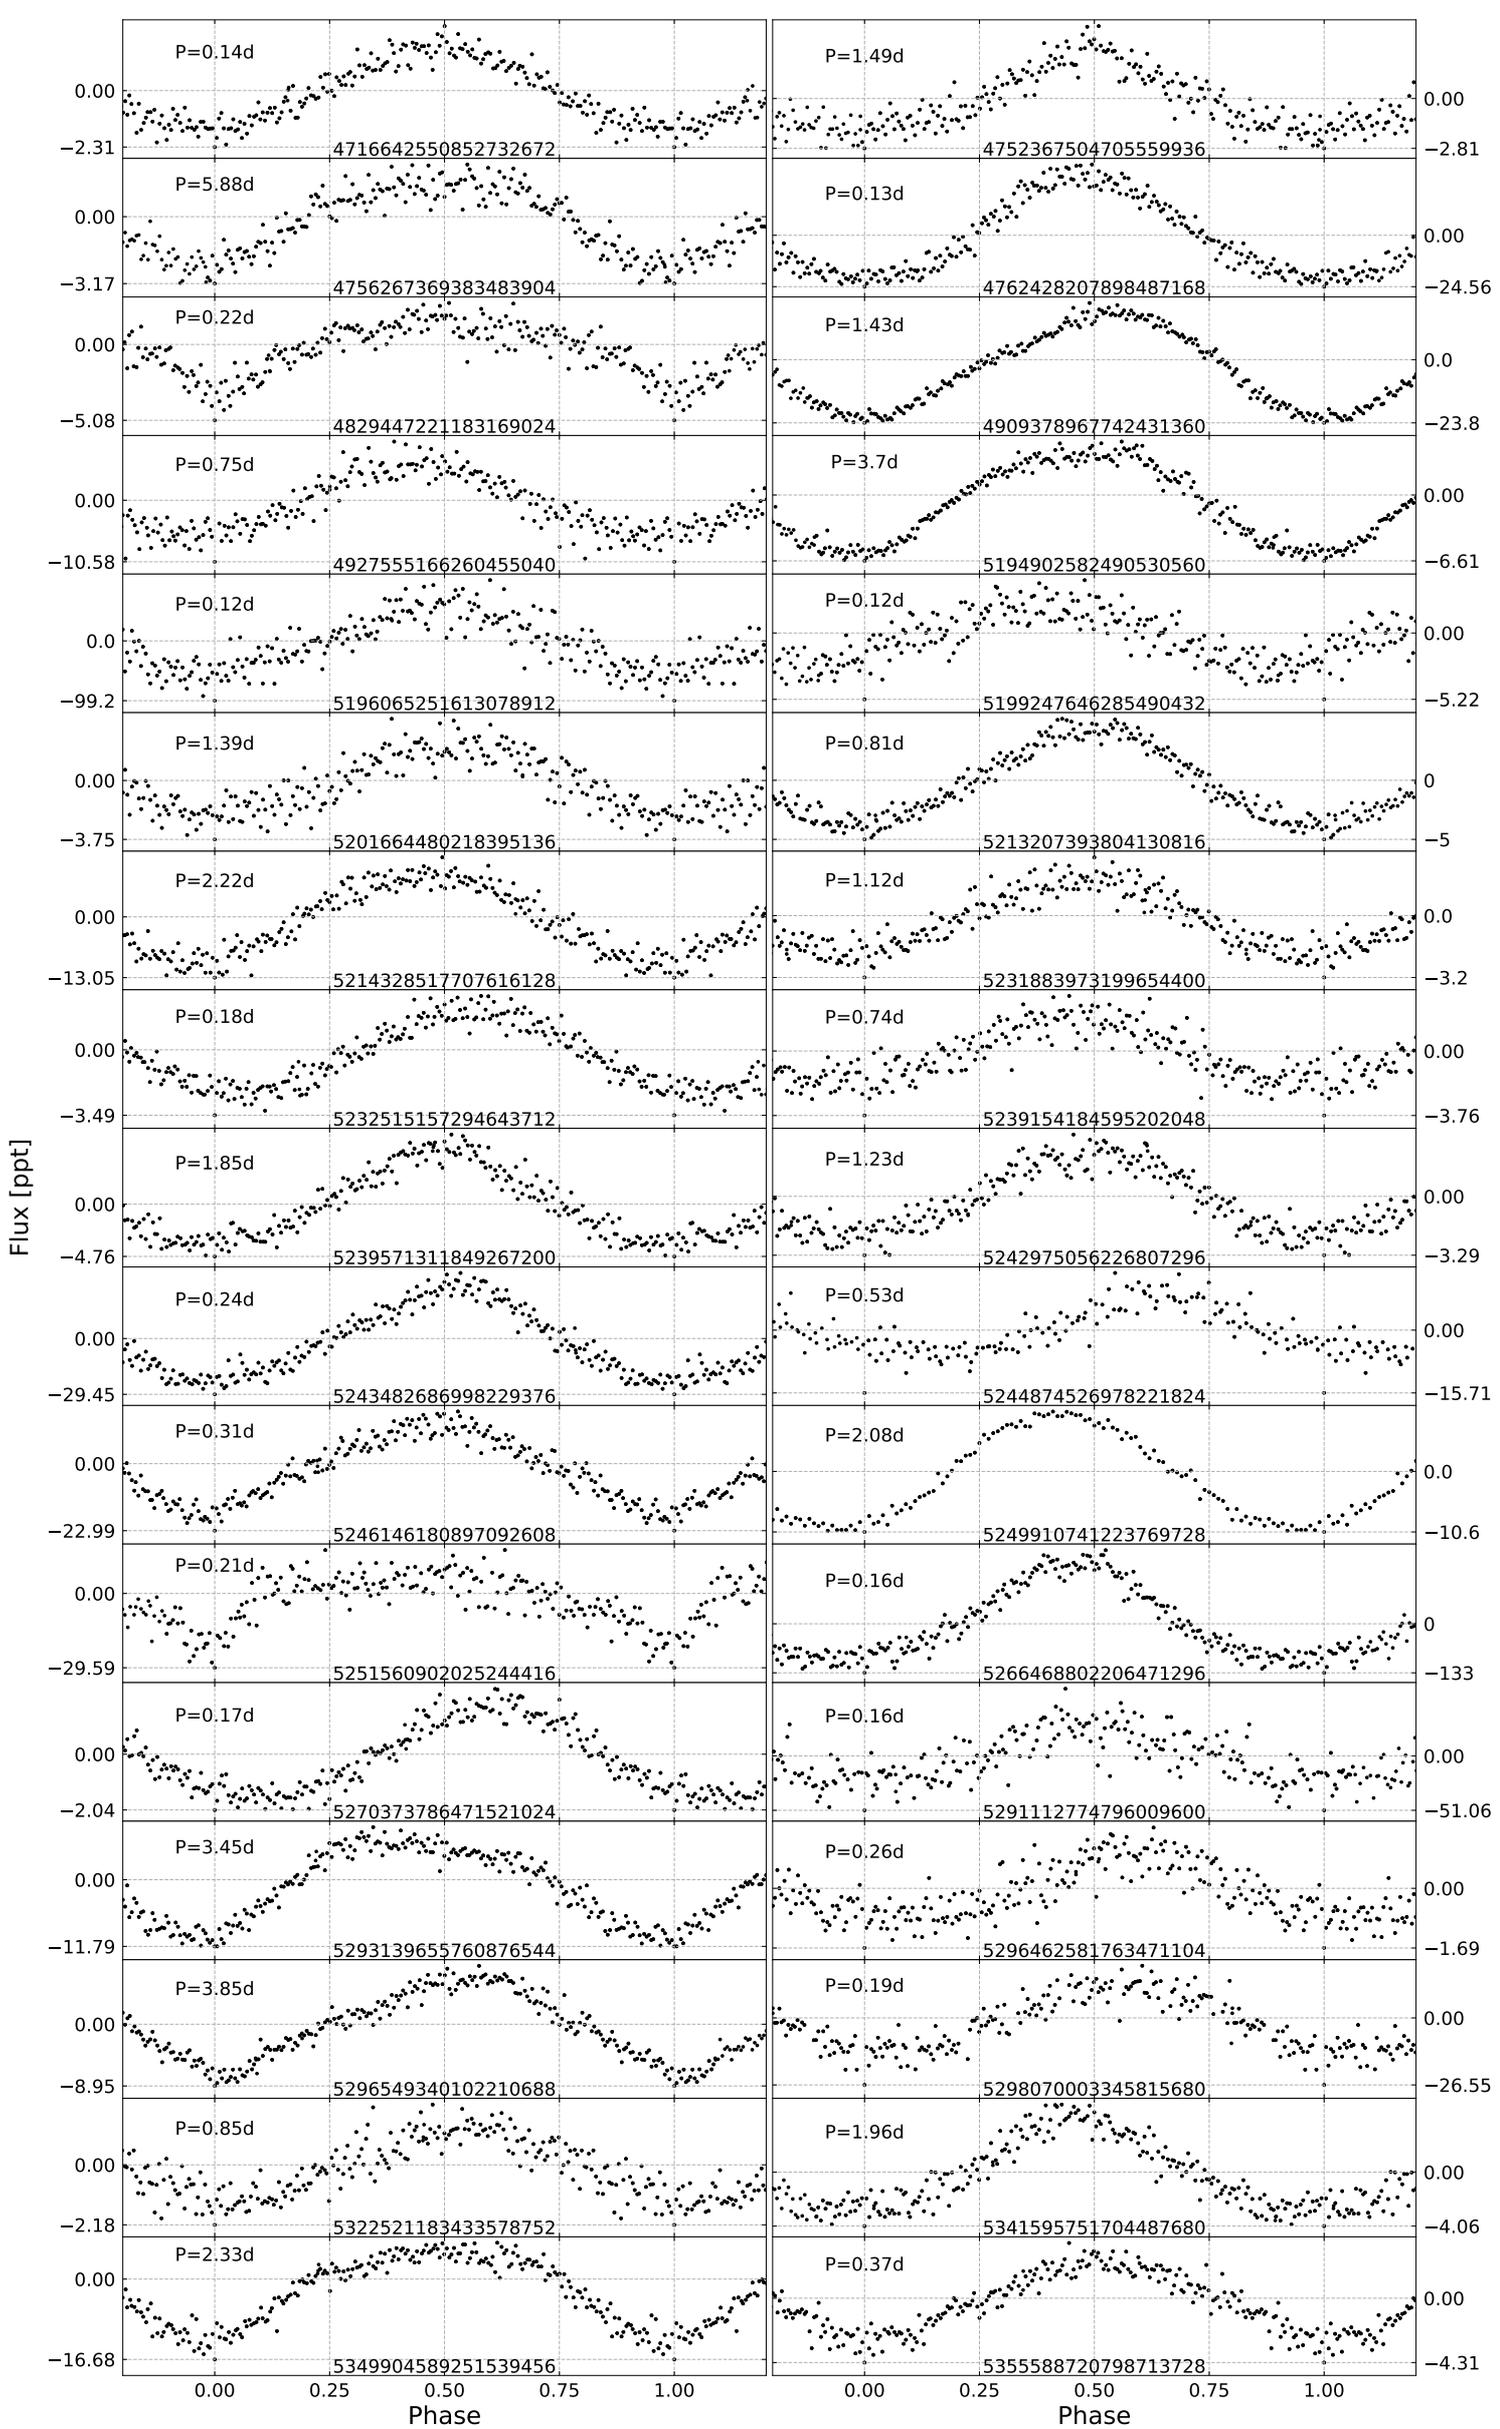

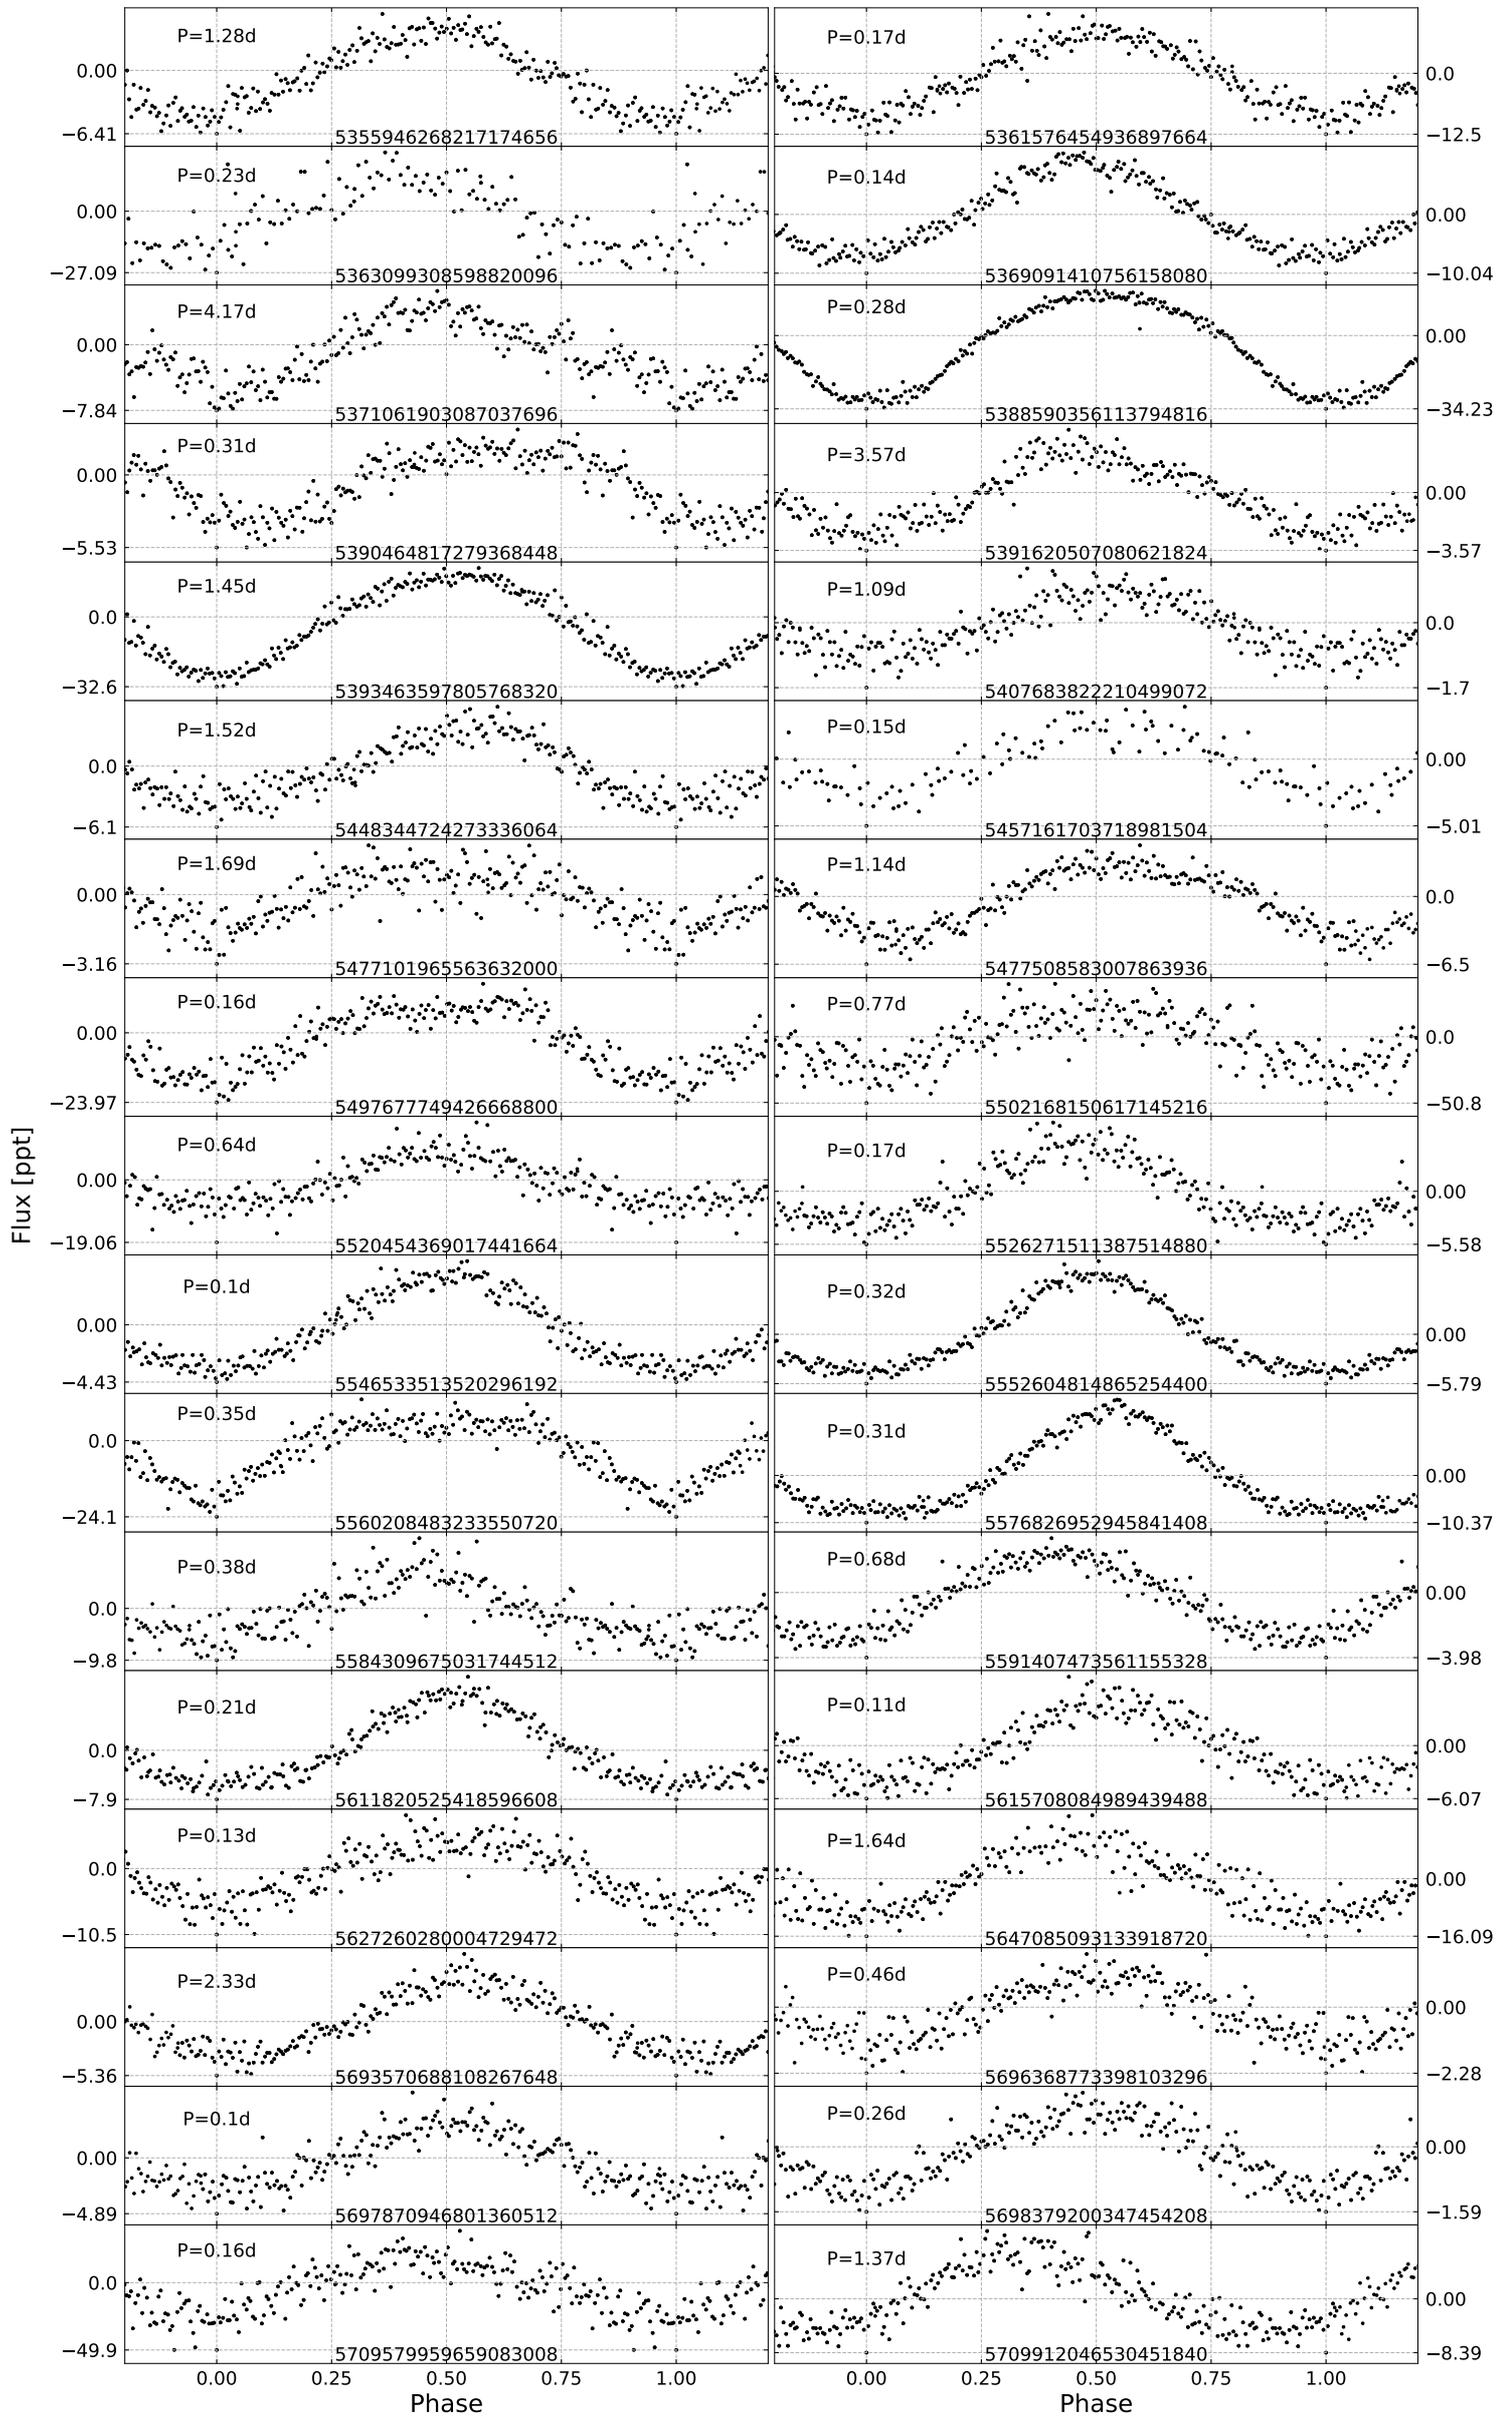

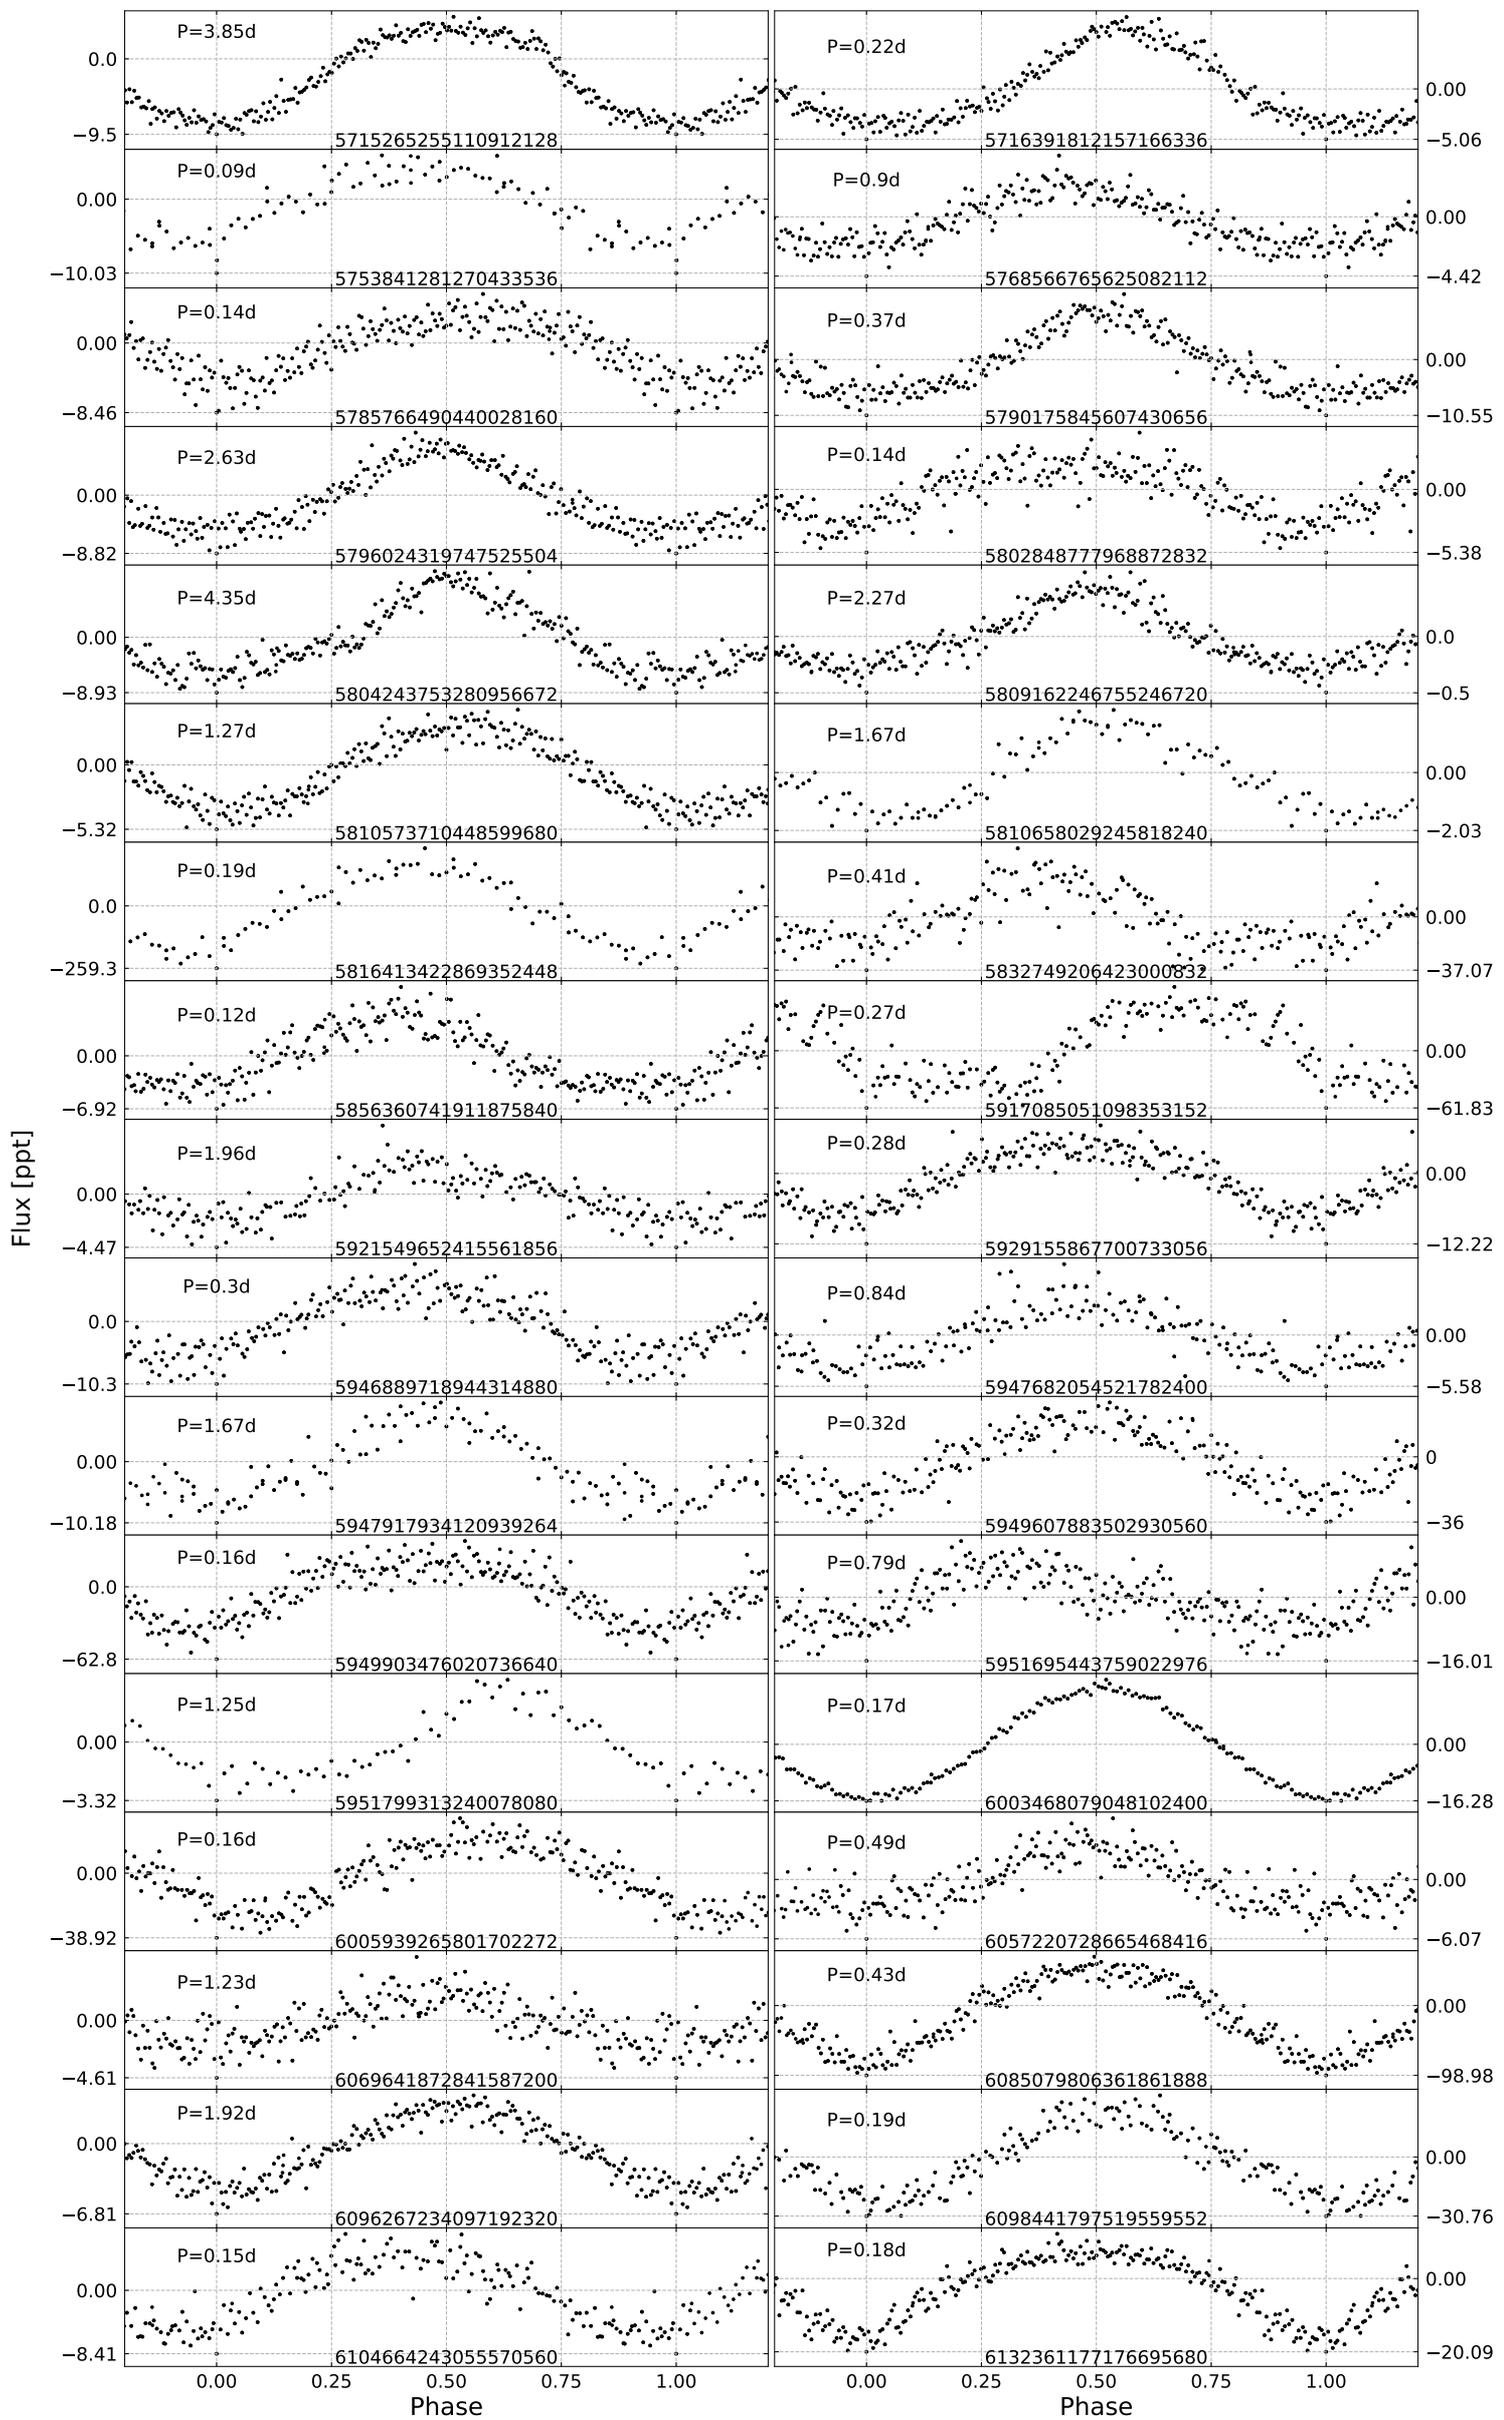

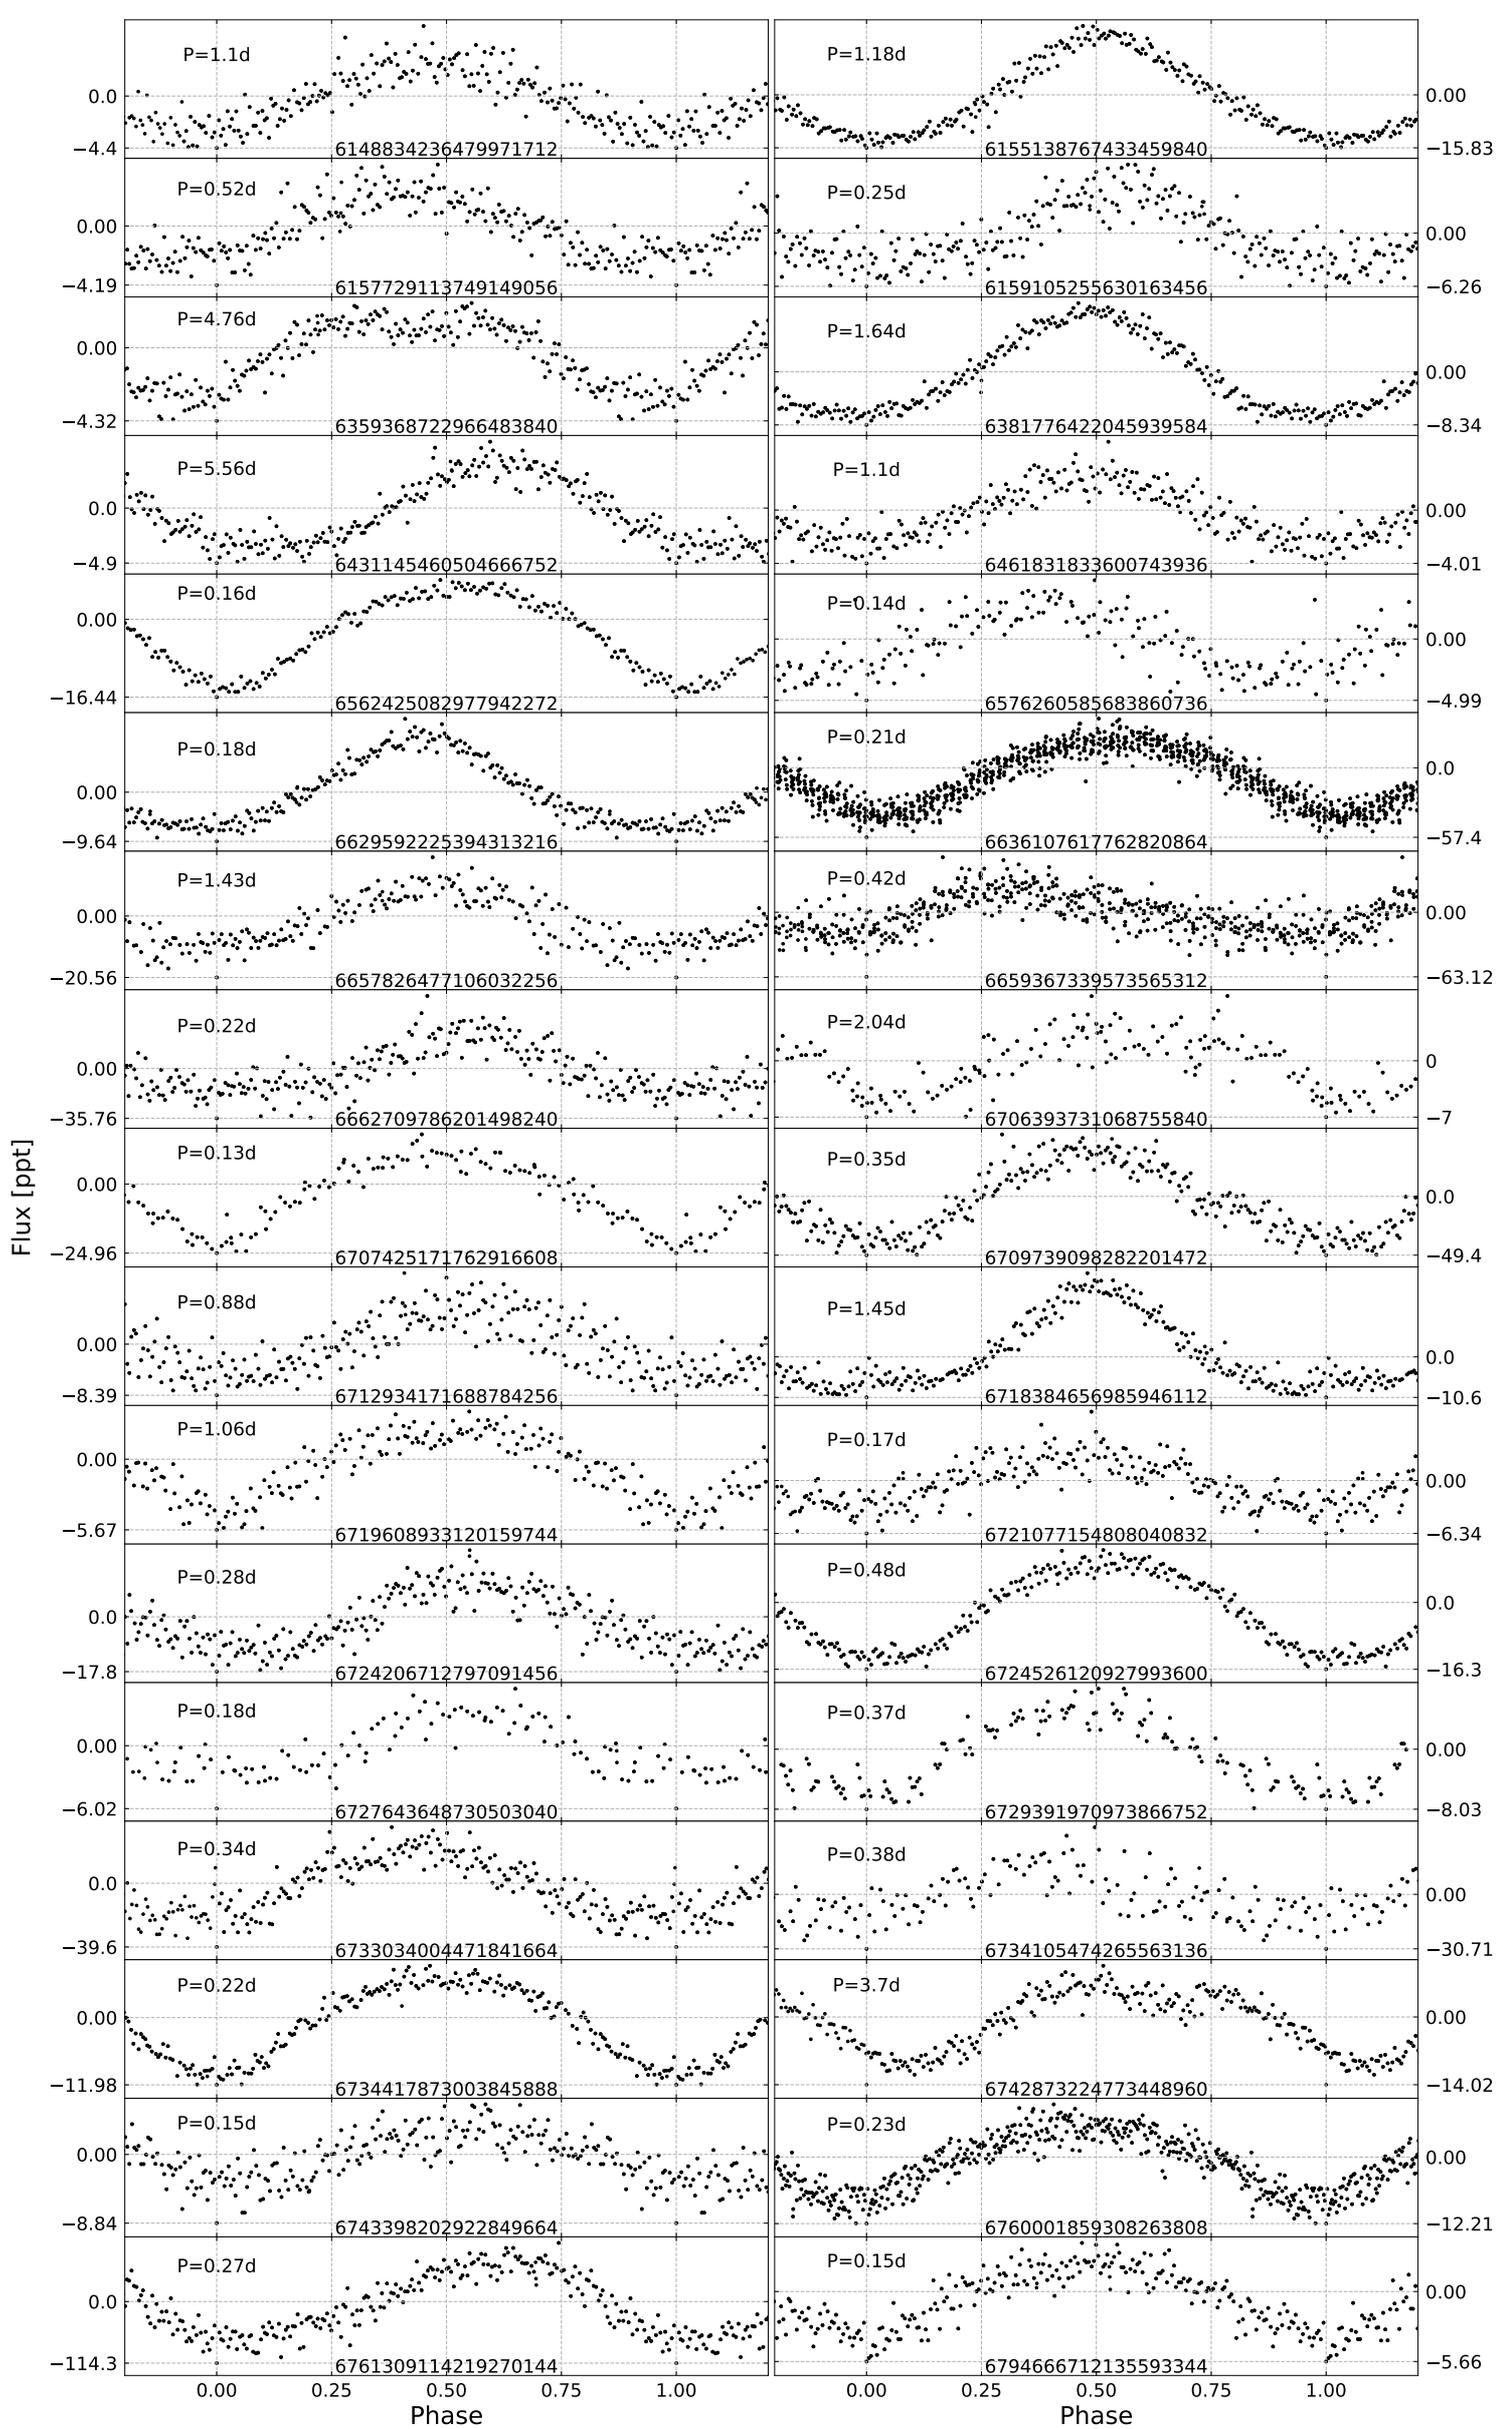

Supplement: Supplementary file 6 [file nospec_phased_1symmetric.pdf]
