# Supplementary material for: A search for variable subdwarf B stars in TESS Full Frame Images -- I. Variable objects in the southern ecliptic hemisphere
Source: arXiv:2011.03465 ancillary file (2020-11-06)

Table 6 and Figure 10 continued...

**Basic information of 31 spectroscopically unclassified variables showing two maxima.  
The table is followed by phased lightcurves of these targets.**

| Gaia DR2            | TIC        | G mag   | Sector     | Period [d] | Remarks                                    |
|---------------------|------------|---------|------------|------------|--------------------------------------------|
| 2909679852999761536 | 33166796   | 14.2988 | 6          | 2.3256     | object 15" away                            |
| 2978115793174302848 | 671282181  | 17.9234 | 5          | 2.1277     | 4 objects within 53"                       |
| 3016508570255997184 | 710301636  | 17.0716 | 6          | 1.2821     | -                                          |
| 3047771538430246784 | 752215680  | 18.3479 | 7          | 1.7544     | crowded field                              |
| 3109216818032728448 | 4999380    | 14.8067 | 7          | 1.389      | crowded field                              |
| 3111794588680353152 | 284124761  | 14.4986 | 7          | 0.6452     | crowded field                              |
| 3236488827993523584 | 713259786  | 16.5284 | 6          | 0.2433     | -                                          |
| 4679135456154867200 | 293218310  | 15.9840 | 2-5,8-9,12 | 0.4367     | -                                          |
| 4714790492235234176 | 231062312  | 13.0713 | 2-3        | 1.6949     | -                                          |
| 4821689823052057728 | 192826669  | 15.7107 | 5-6        | 1.4286     | -                                          |
| 4850445793032736384 | 301050418  | 10.7179 | 3-4        | 1.8182     | -                                          |
| 5219652387372513792 | 304299578  | 15.6212 | 10-11      | 0.2008     | CV ( <a href="#">Halpern et al. 2018</a> ) |
| 5365504803821448576 | 864903758  | 18.0744 | 9-10       | 0.3058     | 3 objects within 21"                       |
| 5365570048662587520 | 864920508  | 18.6547 | 9-10       | 0.3175     | bright object 13" away                     |
| 5366842561574019456 | 938222499  | 18.8956 | 9-10       | 0.3484     | 3 bright objects within 21"                |
| 5429638694292915200 | 4264922    | 12.7556 | 8,9        | 0.0742     | object 17" away                            |
| 5507683266582438528 | 767550400  | 17.4391 | 7-8        | 0.266      | -                                          |
| 5562578205666649088 | 771265934  | 17.3580 | 7          | 0.6245     | object 16" away                            |
| 5815712656008942592 | 1311306525 | 18.0779 | 12         | 0.7519     | 5 objects within 21"                       |
| 5832312223592931072 | 1212826072 | 17.3889 | 12         | 0.5181     | 2 objects within 21"                       |
| 5911440811230926592 | 1510915106 | 18.3779 | 12,13      | 6.25       | 4 objects within 21"                       |
| 5915710764651751936 | 367140246  | 15.8197 | 12         | 0.2519     | UNSW-V 305 18" away                        |
| 5916995406555045760 | 1315155037 | 18.5641 | 12         | 0.4505     | crowded field                              |
| 5946192624280057216 | 1516975280 | 18.1870 | 12         | 0.6849     | crowded field                              |
| 6092765087704842496 | 1050189754 | 16.9423 | 11         | 0.3774     | -                                          |
| 6224708304100799488 | 1176220959 | 17.1617 | 11         | 0.3636     | -                                          |
| 6381526046928596992 | 260824263  | 16.7817 | 1          | 0.5593     | -                                          |
| 6656795070777810688 | 158237390  | 16.3236 | 13         | 2.7778     | object 17" away                            |
| 6732540388160365696 | 151945339  | 15.2134 | 13         | 1.2658     | 6 bright objects within 3'                 |
| 6733697078706189696 | 1823584142 | 17.9054 | 13         | 0.5435     | crowded field                              |
| 6744573756943257472 | 113059781  | 15.8637 | 13         | 1.0424     | 5 bright objects nearby                    |

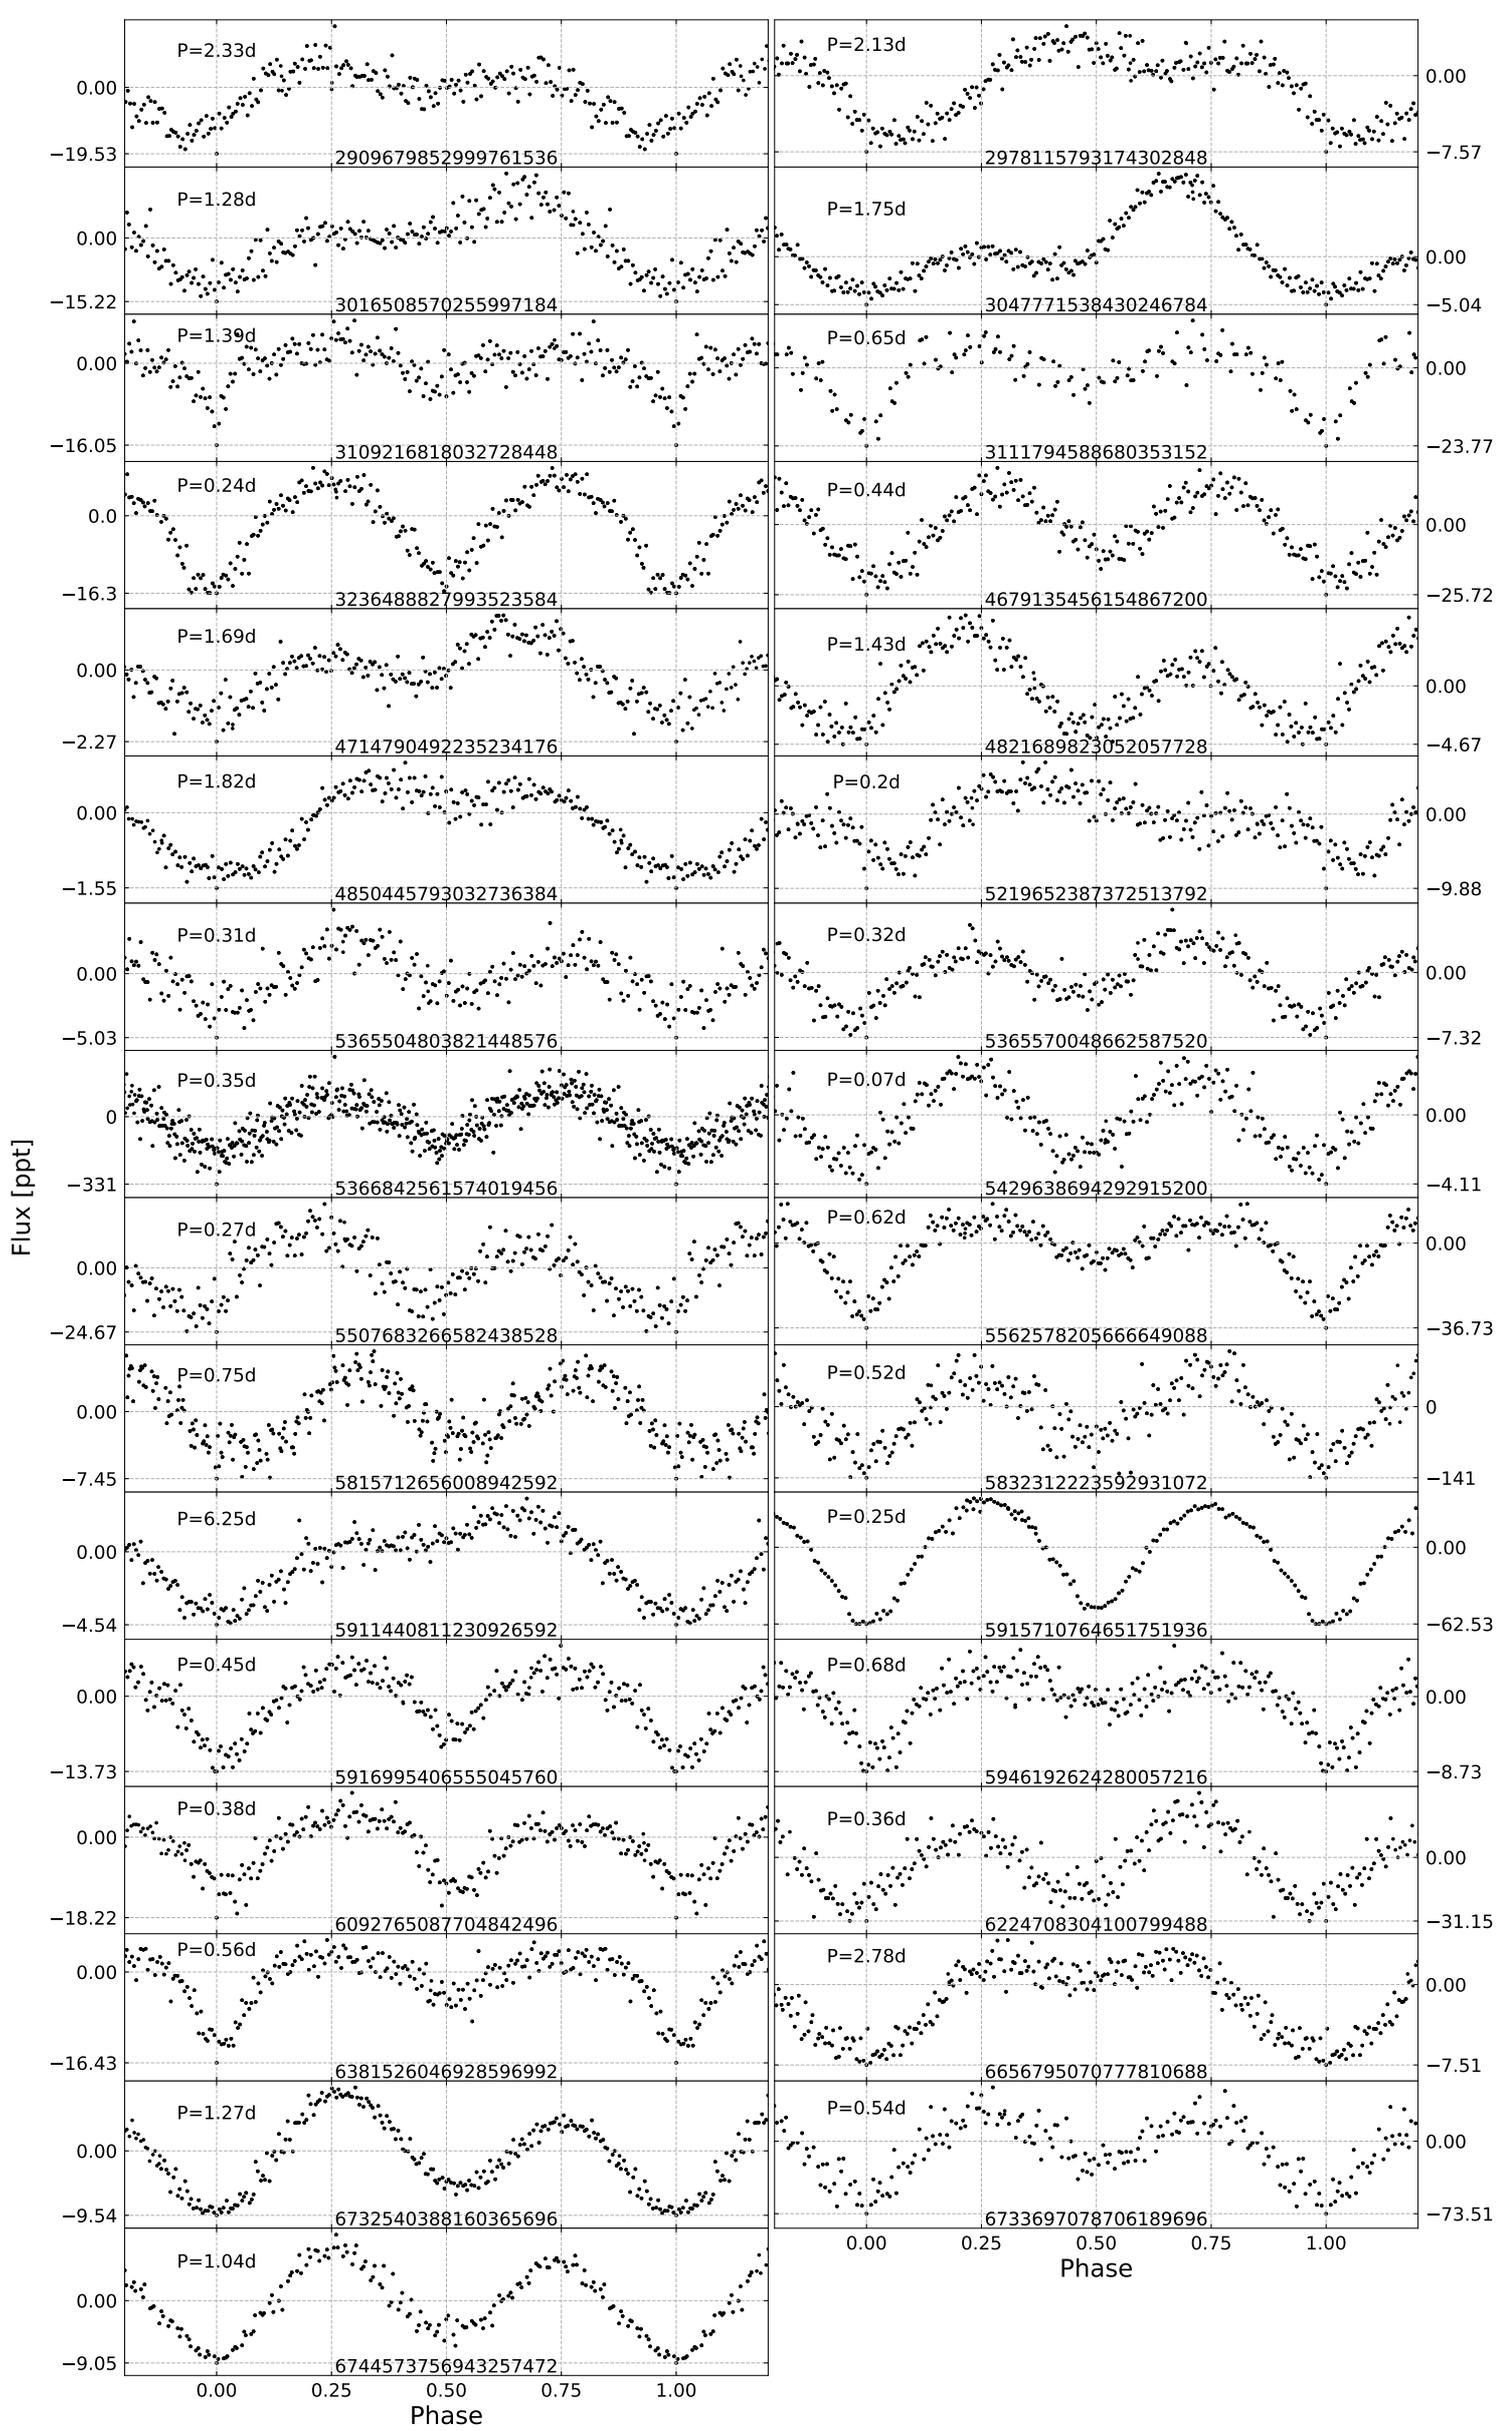

Supplement: Supplementary file 7 [file nospec_phased_2maxima.pdf]
